# Supplementary material for: Faster Sampling without Isoperimetry via Diffusion-based Monte Carlo
Source: arXiv:2401.06325 source file (2024-01-12)
Supplement: Supplementary file 2 [file 0Anotations.tex]

\section{Notations}
\begin{table}[t]
    \centering
    \caption{Notation List}
    \begin{tabular}{c l}
        \toprule
        Symbols & Description\\
        \midrule
        $\varphi_{\sigma^2}$ & The density function of the centered Gaussian distribution, i.e., $\mathcal{N}\left(\vzero,  \sigma^2\mI\right)$. \\
        \midrule
        $p_*, p_{0,0}$ & The target density function (initial distribution of the forward process) \\
        \midrule
        $\left(\rvx_{k,t}\right)_{k\in \mathbb{N}, t\in[0,2\eta]}$ &  The forward process, i.e., SDE~\ref{eq:ps_sde_forward}\\
        $p_{k,t}$ & The density function of $\rvx_{k,t}$, i.e., $\rvx_{k,t}\sim p_{k,t}$\\
        $p_{\infty,0}$ & The density function satisfying $p_{0,0}=p_{0,2\eta}$ when $p_{0,0}=p_{\infty,0}$\\
        \midrule
        $\left(\hat{\rvx}_{k,t}\right)_{k\in \mathbb{N},t\in[0,2\eta]}$ &  The ideal reverse process, i.e., SDE.~\ref{eq:ps_sde_backward_ide}\\
        $\hat{p}_{k,t}$ & The density function of $\hat{\rvx}_t$, i.e., $\hat{\rvx}_t\sim \hat{p}_t$ and $p_t =\hat{p}_{T-t}$\\
        $\hat{P}_t$ & The law of the ideal reverse process SDE.~\ref{eq:ps_sde_backward_ide} over the path space $\mathcal{C}\left([0,2\eta (K+1)]; \R^d\right)$.\\
        \midrule
        $\left(\tilde{\rvx}_{k,t}\right)_{k\in\mathbb{N},t\in[0,T]}$ &  The practical reverse process following from SDE.~\ref{eq:ps_sde_backward_act} with initial distribution $q$\\
        $\tilde{p}_{k,t}$ & The density function of $\tilde{\rvx}_t$, i.e., $\tilde{\rvx}_t\sim \tilde{p}_t$\\
        $\tilde{P}_T$ & The law of the reverse process over the path space $\mathcal{C}\left([0,2\eta (K+1)]; \R^d\right)$.\\
        \midrule
        $\left(\tilde{\rvx}^{p_{K,2\eta}}_{k,t}\right)_{k\in\mathbb{N},t\in[0,T]}$ &  The reverse process following from SDE.~\ref{eq:ps_sde_backward_act} with initial distribution $p_{K,2\eta}$\\
        $\tilde{p}^{p_{K,2\eta}}_{k,t}$ & The density function of $\tilde{\rvx}^{p_{K,2\eta}}_{k,t}$, i.e., $\tilde{\rvx}^{p_{K,2\eta}}_{k,t}\sim \tilde{p}^{p_{K,2\eta}}_{k,t}$\\
        $\tilde{P}^{p_{K,2\eta}}_T$ & The law of the reverse process over the path space $\mathcal{C}\left([0,2\eta (K+1)]; \R^d\right)$.\\
        \bottomrule
    \end{tabular}
    
    \label{tab:notation_list_app}
\end{table}
In this section, we formally formulate the problem and provide detailed notations in Table~\ref{tab:notation_list_app}.

\paragraph{Problem Settings.} We expect to find an algorithm that samples along the backward path of the proximal sampler (PS) proposed by~\citep{chen2022improved} even if the forward path is not explicit.
Specifically, we illustrate the process of PS in Figure~\ref{fig:proximal_sampler_illustration}.
\begin{figure}
    \centering
    \input{0_figs/proof_explain.tex}
    \caption{Proximal Sampler Illustration}
    \label{fig:proximal_sampler_illustration}
\end{figure}
Suppose the initial particle satisfies $\rvx_{0,0}\sim p_{0,0}\propto \exp(-f_*)$.
PS obtains the particle $\rvx_{k,\eta}$ by introducing the transition kernel
\begin{equation}
    \label{eq:den_ps_stage1}
    \mathrm{Pr}\left[\rvx_{k,\eta} | \rvx_{k,0}=\vx_0\right] = \mathcal{N}(\vx_0, \eta \mI),
\end{equation}
and obtain the particle $\rvx_{k,2\eta}$ by introducing
\begin{equation}
    \label{eq:den_ps_stage2}
    p\left(\rvx_{k,2\eta}=\vx | \rvx_{k,\eta}=\vx_\eta\right) \propto \exp\left(-f_{\infty}(\vx)+\frac{1}{2\eta}\left\|\vx - \vx_\eta\right\|^2\right),
\end{equation}
and supposing the restricted Gaussian oracle exists to solve the sampling problem~\ref{eq:den_ps_stage2}.
It should be noted that we have $p_{k,0}=p_{k,2\eta}$ if we suppose $p_{k,0}\propto \exp(-f_\infty)$ due to Lemma~\ref{lem:station_prop_pinfty}.

\paragraph{Derive the Backward Path 1}
To derive the backward path, we should first write the SDE of the forward process.
Actually, the particle update only shows the requirements at time $\eta$ and $2\eta$.
It means any SDE whose transition kernels at time $\eta$ and $2\eta$ are Eq.~\ref{eq:den_ps_stage1} and Eq.~\ref{eq:den_ps_stage2} can be considered as a valid forward process.

Considering the stationary property of $\exp(-f_\infty)$ (Lemma~\ref{lem:station_prop_pinfty}), 
the forward process presented by the following SDE
\begin{equation}
    \label{eq:ps_sde}
    \begin{aligned}
        &\rvx_{k,0} = \rvx_{k-1,2\eta},\quad \mathrm{for}\ k>0, \\
        &\der\rvx_{k, t}=\der B_t, \quad \mathrm{for}\ t\in[0, \eta), \\
        & \der \rvx_{k,t}=\grad \ln p_{\infty,2\eta - t}(\rvx_{k,t})\der t + \der B_t,\quad \mathrm{for}\ t\in[\eta, 2\eta).
    \end{aligned}
\end{equation}
In addition, we set $\rvx_{0,0}\sim p_{0,0}\propto \exp(-f_*)$.
This idea is similar to the proof idea shown in~\cite{chen2022improved}.
For the implementability of the algorithm, we often set $p_{\infty,0}$ to be a Gaussian distribution, i.e., $p_{\infty,0}(\vx)\propto \exp(-\|\vx\|^2/(2c_1))$.
Due to the definition of $p_{\infty,0}$, if we set $\rvx_{0,0}\sim p_{\infty,0}$, with SDE.~\ref{eq:ps_sde}, we have $\rvx_{0,2\eta}\sim p_{\infty,0}$.
This property implies that $p_{\infty,t}$ denotes the probability density function of $\rvx_{0,t}$, and can be presented as
\begin{equation*}
    \begin{aligned}
        p_{\infty,t}(\vx) = (p_{\infty,0} \ast \varphi_{t})(\vx),
    \end{aligned}
\end{equation*}
where $\ast$ denotes the convolution.
It follows from the reverse process derivation in~\citep{cattiaux2021time}.
Both $p_{\infty,0}$ and $\varphi_t$ are high dimensional Gaussian distributions whose density function can be presented as
\begin{equation*}
    \begin{aligned}
        p_{\infty,0}(\vx) = & \left(2\pi c_1\right)^{-d/2}\exp\left(-\frac{\left\|\vx\right\|^2}{2c_1}\right),\\
        \varphi_{t}(\vx) = & \left(2\pi t\right)^{-d/2}\exp\left(-\frac{\left\|\vx\right\|^2}{2t}\right).
    \end{aligned}
\end{equation*}
Hence, the closed form of $p_{\infty, t}$ is 
\begin{equation*}
    \begin{aligned}
        p_{\infty,t}(\vx) = & \int_{\vv\in\R^d} (2\pi c_1)^{-d/2} \exp \left(-\frac{\left\|\vv\right\|^2}{2c_1}\right)\cdot (2\pi t)^{-d/2}\exp\left(-\frac{\left\|\vx-\vv\right\|^2}{2t}\right) \der\vv\\
        = & (2\pi c_1)^{-d/2} \cdot (2\pi t)^{-d/2} \int_{\vv\in\R^d}\exp\left(-\frac{\left\|\vv\right\|^2}{2c_1} - \frac{\left\|\vx\right\|^2-2\vx^\top\vv + \left\|\vv\right\|^2}{2t}\right) \der \vv\\
        = & (2\pi c_1)^{-d/2} \cdot (2\pi t)^{-d/2} \cdot \exp\left(-\frac{\left\|\vx\right\|^2}{2t+2c_1}\right)\\
        & \int_{\vv\in\R^d}\exp\left(-\left(\frac{1}{2t}+\frac{1}{2c_1}\right)\left\|\vv\right\|^2 + \frac{1}{t}\vx^\top\vv-\frac{(2t)^{-2}}{(2t)^{-1}+ (2c_1)^{-1}}\left\|\vx\right\|^2\right) \der\vv\\
        =& (2\pi (t+c_1))^{-d/2}\exp\left(-\frac{\left\|\vx\right\|^2}{2(t+c_1)}\right).
    \end{aligned}
\end{equation*}
and 
\begin{equation}
    \grad \ln p_{\infty, t}(\vx) = -(t+c_1)^{-1}\vx. 
\end{equation}
In this condition, we can rewrite SDE.~\ref{eq:ps_sde} as
\begin{equation}
    \label{eq:ps_sde_exp}
    \begin{aligned}
        &\rvx_{k,0} = \rvx_{k-1,2\eta},\quad \mathrm{for}\ k>0, \\
        &\der\rvx_{k, t}=\der B_t, \quad \mathrm{for}\ t\in[0, \eta), \\
        & \der \rvx_{k,t}=-(2\eta -t+c_1)\rvx_{k,t}\der t + \der B_t,\quad \mathrm{for}\ t\in[\eta, 2\eta).
    \end{aligned}
\end{equation}
For calculation convenience, we introduce the auxiliary random variable $\dot{\rvx}_{k,t}=\rvx_{k,t+\eta}$ for $t\in[0,\eta)$.
Then, the SDE of $\dot{\rvx}_{k,t}$ is 
\begin{equation*}
    \der \dot{\rvx}_{k,t}=-(\eta-t+c_1)\dot{\rvx}_{k,t}\der t + \der B_t,
\end{equation*}
which is an OU process whose solution has an explicit form shown in~\citep{2016Degradation}.
With similar notations, we define
\begin{equation*}
    \alpha(t,s)= -\int_s^t -(\eta - u+c_1)\der u = (\eta+c_1)(t-s)+\frac{s^2}{2}-\frac{t^2}{2},
\end{equation*}
then we have
\begin{equation*}
    \begin{aligned}
        \dot{\rvx}_{k,t} = & e^{-\alpha(t,0)}\left[\dot{\rvx}_{k,0} + \int_0^t e^{\alpha(s,0)}\der B_s\right]= e^{-\alpha(t,0)}\dot{\rvx}_{k,0}+ \mathcal{N}\left(0, \int_0^t e^{2(\alpha(s,0)-\alpha(t,0))}\der s\right)\\
        = & e^{-\alpha(t,0)}\dot{\rvx}_{k,0}+ \mathcal{N}\left(0, \int_0^t \exp\left(2(\eta+c_1)(s-t)-s^2 + t^2\right)\der s\right).
    \end{aligned}
\end{equation*}
It means the solution of $\dot{\rvx}_{k,t}$ will contain the error function, which can hardly be obtained precisely.
That means the exact transition kernel of SDE.~\ref{eq:ps_sde_exp} can hardly be calculated when $t\in[\eta,2\eta)$, and the backward path cannot be obtained.

\begin{figure}
    \centering
    \input{0_figs/process_explain_2}
    \caption{Proximal Sampler Illustration}
    \label{fig:proximal_sampler_illustration_2}
\end{figure}

\paragraph{Derive the Backward Path 2}
Similar to the previous paragraph, we also need to consider the forward process first.
For the particles' update of the first stage, the transition kernel Eq.~\ref{eq:den_ps_stage1} corresponds to the 
the following SDE at time $\eta$
\begin{equation*}
    \label{eq:sde_stage1}
    \begin{aligned}
        &\rvx_{k,0} = \rvx_{k-1, 2\eta}\quad \mathrm{for}\ k>0,\\
        &\der \rvx_{k,t}=\der B_t\quad \mathrm{for}\ t\in[0,\eta).
    \end{aligned}
\end{equation*}
Considering the second stage, we require the SDE at time $\eta$ to have the transition kernel Eq.~\ref{eq:den_ps_stage2}, i.e.,
\begin{equation*}
    \begin{aligned}
        p(\vx_\eta, \eta|\vx_0, 0) = C_\eta \exp\left(-f_\infty(\vx_\eta)-\frac{\left\|\vx_\eta-\vx_0\right\|^2}{2\eta}\right)= \frac{\exp\left(-f_\infty(\vx_\eta)-\frac{\left\|\vx_\eta-\vx_0\right\|^2}{2\eta}\right)}{\int \exp\left(-f_\infty(\vz)-\frac{\left\|\vz-\vx_0\right\|^2}{2\eta}\right) \der \vz}. \\
    \end{aligned}
\end{equation*}
For a tractable forward process, we suppose $f_\infty(\vx)=c_0\left\|\vx\right\|^2$.
In this condition, the transition kernel can be reformulated as
\begin{equation*}
    \begin{aligned}
        p(\vx_\eta, \eta|\vx_0, 0) = &\frac{\exp\left(-c_0\left\|\vx_\eta\right\|^2-\frac{\left\|\vx_\eta-\vx_0\right\|^2}{2\eta}\right)}{\int \exp\left(-c_0\left\|\vz\right\|^2-\frac{\left\|\vz-\vx_0\right\|^2}{2\eta}\right) \der \vz}= \frac{\exp\left(-c_0\left\|\vx_\eta\right\|^2-\frac{\left\|\vx_\eta\right\|^2}{2\eta}+ \frac{\vx_\eta^\top \vx_0}{\eta}-\frac{\left\|\vx_0\right\|^2}{2\eta}\right)}{\int \exp\left(-c_0\left\|\vz\right\|^2-\frac{\left\|\vz\right\|^2}{2\eta}+\frac{z^\top \vx_0}{\eta}-\frac{\left\|\vx_0\right\|^2}{2\eta}\right) \der \vz}\\
        = & \frac{\exp\left(-\left(c_0+\frac{1}{2\eta}\right)\left\|\vx_\eta-\frac{\vx_0}{2\eta c_0+1}\right\|^2-\frac{c_0 \left\|\vx_0\right\|^2}{2\eta c_0+1}\right)}{\int \exp\left(-\left(c_0+\frac{1}{2\eta}\right)\left\|\vz-\frac{\vx_0}{2\eta c_0+1}\right\|^2-\frac{c_0\left\|\vx_0\right\|^2}{2\eta c_0+1}\right) \der \vz}\\
        = & \frac{\exp\left(-\left(c_0+\frac{1}{2\eta}\right)\left\|\vx_\eta-\frac{\vx_0}{2\eta c_0+1}\right\|^2\right)}{\int\exp\left(-\left(c_0+\frac{1}{2\eta}\right)\left\|\vz-\frac{\vx_0}{2\eta c_0+1}\right\|^2\right) \der \vz} \propto \exp\left(-\left(c_0+\frac{1}{2\eta}\right)\left\|\vx_\eta-\frac{\vx_0}{2\eta c_0+1}\right\|^2\right).
    \end{aligned}
\end{equation*}
Then, we consider the normalizing constant of this transition kernel.
Considering that $p(\vx_\eta, \eta|\vx_0, 0)$ is a Gaussian distribution, and can be simplified as
\begin{equation*}
    \begin{aligned}
        p(\vx_\eta, \eta|\vx_0, 0) \propto & \exp\left(-\left(c_0+\frac{1}{2\eta}\right)\left\|\vx_\eta-\frac{\vx_0}{2\eta c_0+1}\right\|^2\right)\\
        = & \exp\left(- \frac{\left\|\vx_\eta-\frac{\vx_0}{2\eta c_0+1}\right\|^2}{\frac{1}{\left(c_0+\frac{1}{2\eta}\right)}}\right) = \exp\left(- \frac{\left\|\vx_\eta-\frac{\vx_0}{2\eta c_0+1}\right\|^2}{2\cdot \frac{\eta}{2\eta c_0+1}}\right)
    \end{aligned}
\end{equation*}
whose mean and variance are
\begin{equation*}
    \vm = \frac{\vx_0}{2\eta c_0 +1}\quad \mathrm{and}\quad \Sigma = \frac{\eta}{2\eta c_0 +1}\mI.
\end{equation*}
Hence, we have
\begin{equation}
    \label{eq:transition_kernel_eta}
    p(\vx_\eta, \eta|\vx_0, 0) = \left(2\pi \cdot \frac{\eta}{2\eta c_0 +1}\right)^{-\frac{d}{2}}\cdot \exp\left(- \frac{\left\|\vx_\eta-\frac{\vx_0}{2\eta c_0+1}\right\|^2}{2\cdot \frac{\eta}{2\eta c_0+1}}\right).
\end{equation}
We try to find an OU process with time-independent drift and diffusion terms, whose transition kernel at time $\eta$ is Eq.~\ref{eq:transition_kernel_eta}.
With the method of undetermined coefficients, suppose the OU process is 
\begin{equation*}
    \begin{aligned}
        &\dot{\rvx}_{k,0} = \rvx_{k,\eta}\\
        &\der\dot{\rvx}_{k,t} = -\theta \dot{\rvx}_{k,t}\der t + \sigma \der B_t.
    \end{aligned}
\end{equation*}
According to the Fokker-Plancker equation, the dynamics of its probability density function will be
\begin{equation*}
    \frac{\partial \dot{p}}{\partial t} = \nabla \cdot \left(\dot{p}\theta \vx\right) + \frac{\sigma^2}{2}\Delta \dot{p}. 
\end{equation*}
In this condition, the mean and variance of $\dot{\rvx}_{k,\eta}$ will be 
\begin{equation*}
    \dot{\vm} = e^{-\theta \eta}\cdot \vx_{0}\quad \mathrm{and}\quad \dot{\Sigma} = \frac{\sigma^2}{2\theta}\cdot \left(1-e^{-2\theta\eta}\right)\mI
\end{equation*}
when $\dot{\rvx}_{k,0}=\vx_0$.
We require
\begin{equation*}
    \left\{
        \begin{aligned}
            & e^{-\theta\eta} =\frac{1}{2\eta c_0 +1}\\
            & \frac{\sigma^2}{2\theta}\cdot \left(1-e^{-2\theta\eta}\right) = \frac{\eta}{2\eta c_0 +1}
        \end{aligned}
    \right. \Rightarrow 
    \left\{
        \begin{aligned}
            \theta = & \frac{\ln(2\eta c_0+1)}{\eta}\\
        \sigma = & \sqrt{\frac{(2\eta c_0+1)\ln(2\eta c_0 +1)}{2\eta c_0 (\eta c_0 +1)}}
        \end{aligned}
    \right. ,
\end{equation*}
where the choice of $\sigma$ follows from the following equation
\begin{equation*}
    \begin{aligned}
        &\frac{\sigma^2}{2\theta} \cdot \left(1-e^{-2\theta\eta}\right) = \frac{\sigma^2}{2\theta}\cdot \left(1-\left(2\eta c_0+1\right)^{-2}\right) = \frac{\eta}{2\eta c_0 +1}\\
        \Leftrightarrow\quad & \frac{\sigma^2}{2\theta} \cdot \frac{4\eta^2c_0^2+4\eta c_0}{(2\eta c_0+1)^2} = \frac{\eta}{2\eta c_0+1}\\
        \Leftrightarrow\quad &\frac{\sigma^2}{2\theta} = \frac{\eta}{2\eta c_0 + 1}\cdot \frac{(2\eta c_0+1)^2}{4\eta^2c_0^2 + 4\eta c_0} =\frac{2\eta c_0 +1}{4\eta c_0^2 + 4 c_0}\\
        \Rightarrow\quad  & \sigma = \sqrt{\frac{2\eta c_0+1}{2\eta c_0^2 + 2c_0}\cdot \theta} =\sqrt{\frac{(2\eta c_0+1)\ln(2\eta c_0 +1)}{2\eta c_0 (\eta c_0 +1)}}.
    \end{aligned}
\end{equation*}
We summarize the SDE of the forward process can be
\begin{equation}
    \label{eq:ps_sde_rev}
    \begin{aligned}
        &\rvx_{k,0} = \rvx_{k-1,2\eta},\quad \mathrm{for}\ k>0, \\
        &\der\rvx_{k, t}=\der B_t, \quad \mathrm{for}\ t\in[0, \eta), \\
        & \der \rvx_{k,t}=-\frac{\ln(2\eta c_0+1)}{\eta} \rvx_{k,t}\der t + \sqrt{\frac{(2\eta c_0+1)\ln(2\eta c_0 +1)}{2\eta c_0 (\eta c_0 +1)}} \der B_t,\quad \mathrm{for}\ t\in[\eta, 2\eta).
    \end{aligned}
\end{equation}
For simple notations, we define
\begin{equation*}
    \dot{D} = \frac{\sigma^2}{2} = \frac{(2\eta c_0+1)\ln (2\eta c_0+1)}{4\eta c_0 (\eta c_0 +1)}.
\end{equation*}
Then, the transition kernel of SDE.~\ref{eq:ps_sde_rev} when $t\in[\eta,2\eta)$ satisfies
\begin{equation*}
    \begin{aligned}
        p(\rvx_{k,t}=\vx_{t}, t | \rvx_{k,\eta}=\vx_\eta, \eta) = & \left(2\pi\cdot \frac{\dot{D}}{\theta}\cdot \left(1-e^{-2\theta (t-\eta)}\right)\right)^{-\frac{d}{2}}\cdot \exp\left(-\frac{\left\|\vx_t - e^{-\theta (t-\eta)}\vx_\eta\right\|^2}{2\cdot \frac{\dot{D}(1-e^{-2\theta (t-\eta)})}{\theta}}\right)
    \end{aligned}
\end{equation*}
whose mean and variance are
\begin{equation*}
    \begin{aligned}
        \vm_t & = e^{-\theta(t-\eta)}\vx_\eta = \exp\left(-\frac{\ln(2\eta c_0+1)}{\eta}\cdot (t-\eta)\right) \vx_\eta= \left(2\eta c_0+1\right)^{\frac{\eta -t}{\eta}}\vx_\eta\\
        \Sigma_t & = \frac{\dot{D}}{\theta}\left(1-e^{-2\theta(t-\eta)}\right)\mI = \frac{2\eta c_0+1}{4\eta c_0 + 4c_0}\cdot \left[1-(2\eta c_0+1)^{\frac{2(\eta-t)}{\eta}}\right]\mI.
    \end{aligned}
\end{equation*}
It means that, when $t\in[\eta,2\eta]$, we have
\begin{equation*}
    p_{k,t}(\vx_t) = \int p_{k,\eta}(\vx_\eta)\cdot p(\rvx_{k,t}=\vx_{t}, t | \rvx_{k,\eta}=\vx_\eta, \eta) \der \vx_\eta. 
\end{equation*}
With the explicit forward process, i.e., SDE.~\ref{eq:ps_sde_rev}, we start to consider its backward path.
Suppose $\rvx_{k, 2\eta}=\hat{\rvx}_{k,0}$ is given and $t\in[0, \eta] $, we have the following reverse SDE
\begin{equation*}
    \begin{aligned}
        \der \hat{\rvx}_{k,t} =\left[ \frac{\ln (2\eta c_0+1)}{\eta} \cdot \hat{\rvx}_{k,t} + \frac{(2\eta c_0+1)\ln(2\eta c_0 +1)}{2\eta c_0 (\eta c_0+1)}\grad \ln p_{k,2\eta -t}(\hat{\rvx}_{k,t})\right]\der t + \sqrt{\frac{(2\eta c_0+1)\ln(2\eta c_0 +1)}{2\eta c_0 (\eta c_0+1)}}\der B_t.
    \end{aligned}
\end{equation*}
\begin{framed}
    \centering
    If we consider constructing a diffusion model with the forward process SDE.~\ref{eq:ps_sde_rev}, we should only parameterize $\grad \ln p_{k,2\eta-t}(\vx)$ just as that in traditional diffusion models.
\end{framed}
In the previous analysis of the backward path, we utilize $\grad \ln p_{k, 2\eta}$ to approximate $\grad \ln p_{k, 2\eta-t}$ for the simple implementation.
While we defer the discretization operation and consider the implementation of $\grad \ln p_{k,2\eta-t}$.
With the transition kernel, we have
\begin{equation*}
    \begin{aligned}
        \grad \ln p_{k, 2\eta - t}(\vx) = & \frac{\grad p_{k,2\eta -t}(\vx)}{p_{k,2\eta -t}(\vx)} = \frac{\int p_{k,\eta}(\vx_\eta) \grad p(\rvx_{k,2\eta-t}=\vx, 2\eta-t | \rvx_{k,\eta}=\vx_\eta, \eta)\der \vx_\eta}{\int p_{k,\eta}(\vx_\eta)\cdot p(\rvx_{k,2\eta-t}=\vx, 2\eta-t | \rvx_{k,\eta}=\vx_\eta, \eta) \der \vx_\eta }\\
        = & \frac{\int p_{k,\eta}(\vx_\eta)\exp\left[-\frac{\left\|\vx - (2\eta c_0+1)^{(t-\eta)/\eta}\vx_\eta\right\|^2}{2\Sigma_{2\eta -t}}\right]\cdot \left(-\frac{\vx-(2\eta c_0+1)^{(t-\eta)/\eta}\vx_\eta}{\Sigma_{2\eta -t}}\right)\der \vx_\eta}{\int p_{k,\eta}(\vx_\eta)\exp\left[-\frac{\left\|\vx - (2\eta c_0+1)^{(t-\eta)/\eta}\vx_\eta\right\|^2}{2\Sigma_{2\eta -t}}\right] \der \vx_\eta}.
    \end{aligned}
\end{equation*}
It can be reformulated as
\begin{equation*}
     \begin{aligned}
         &\grad \ln p_{k, 2\eta - t}(\vx)= \mathbb{E}_{\rvx_\eta\sim q_{k,2\eta - t}(\cdot|\vx)}\left[\frac{(2\eta c_0+1)^{(t-\eta)/\eta}\vx_\eta-\vx}{\Sigma_{2\eta -t}}\right] \\
        \quad\mathrm{s.t.}\quad &q_{k,2\eta - t}(\vy|\vx)\propto p_{k,\eta}(\vy)\cdot \exp\left[-\frac{\left\|\vx - (2\eta c_0+1)^{(t-\eta)/\eta}\vy\right\|^2}{2\Sigma_{2\eta -t}}\right].
     \end{aligned}
\end{equation*}
That means obtaining $\grad\ln p_{k,2\eta - t}$ is equivalent to sample from $q_{k,2\eta -t}$ where $q_{k,2\eta -t}$ has good properties.
For example, if we approximate $\grad\ln p_{k,2\eta - t}$ with $\grad \ln p_{k,2\eta}$ when $t\in [0,\eta]$, then we have
\begin{equation*}
    q_{k,2\eta}(\vy|\vx) = p_{k,\eta}(\vy) \cdot \exp\left(-\frac{\left\|\vx - \frac{1}{2\eta c_0+1}\vy\right\|^2}{2\cdot \frac{\eta}{2\eta c_0+1}}\right).
\end{equation*}
Suppose the smoothness of $p_{k,\eta}$ can be controlled and $\eta$ is small enough, $q_{k,2\eta}(\vy|\vx)$ will be a strongly log-concave density function.
To sample from $q_{k,2\eta}(\vy|\vx)$, the key point is to obtain $\grad_{\vy}\ln q_{k,2\eta}(\vy|\vx)$, due to the following equation,
\begin{equation*}
    \grad \ln q_{k,2\eta}(\vy|\vx) = \grad\ln p_{k,\eta}(\vy) + \grad_{\vy} \left(-\frac{\left\|\vx - \frac{1}{2\eta c_0+1}\vy\right\|^2}{2\cdot \frac{\eta}{2\eta c_0+1}}\right),
\end{equation*}
where the latter term has a closed form. 
Hence, the bottleneck is to obtain $\grad\ln p_{k,\eta}$. 
In the following, we introduce a recursive method to obtain $\grad\ln p_{k,\eta}$.
According to the proximal sampler algorithms, we have
\begin{equation*}
    \begin{aligned}
        & p_{k,\eta}(\vx) = \int p_{k,0}(\vy)\cdot  (2\eta \pi)^{-\frac{d}{2}}\exp\left[\frac{-\left\|\vx -\vy\right\|^2}{2\eta}\right]\der\vy\\
        \Rightarrow\quad & \grad\ln p_{k,\eta}(\vx) = \frac{\int p_{k,0}(\vy)\cdot  (2\eta \pi)^{-\frac{d}{2}}\exp\left[\frac{-\left\|\vx -\vy\right\|^2}{2\eta}\right]\cdot \left(- \frac{\vx-\vy}{\eta}\right)\der\vy}{\int p_{k,0}(\vy)\cdot  (2\eta \pi)^{-\frac{d}{2}}\exp\left[\frac{-\left\|\vx -\vy\right\|^2}{2\eta}\right]\der\vy}.
    \end{aligned}
\end{equation*}
Similarly, it can also be reformulated as
\begin{equation*}
    \begin{aligned}
        &\grad \ln p_{k,\eta}(\vx) = \mathbb{E}_{\rvy\sim q_{k,\eta}(\cdot|\vx)}\left[\frac{\rvy - \vx}{\eta}\right]\\
        \mathrm{s.t.} \quad & q_{k,\eta}(\vy|\vx) \propto p_{k,0}(\vy)\cdot \exp\left(-\frac{\left\|\vx-\vy\right\|^2}{2\eta}\right) 
    \end{aligned}.
\end{equation*}
In order to calculate the gradient complexity of the recursive method, we informally have the following logic
\begin{equation*}
    \begin{aligned}
        \mathrm{To\ obtain\ }\grad\ln p_{k,2\eta}(\vx) \xLeftarrow{\mathrm{sample\ number\ controlled\ by\ concentration}} \mathrm{Sample\ from\ }q^\prime_{k,2\eta}\mathrm{\ approximating\ }q_{k,2\eta}(\vx_1|\vx)\\
        \xLeftarrow{\mathrm{approximate\ error\ controlled\ by\ iteration\ number\ of\ ULA}} \mathrm{To\ obtain\ }\grad\ln p_{k,\eta}(\vx_1)\\
        \xLeftarrow{\mathrm{sample\ number\ controlled\ by\ concentration}} \mathrm{Sample\ from\ }q^\prime_{k,\eta}\mathrm{\ approximating\ }q_{k,\eta}(\vx_2|\vx_1)\\
        \xLeftarrow{\mathrm{approximate\ error\ controlled\ by\ iteration\ number\ of\ ULA}} \mathrm{To\ obtain\ }\grad\ln p_{k,0}(\vx_2)=\grad \ln p_{k-1,2\eta}(\vx_2).
    \end{aligned}
\end{equation*}
We summarize the algorithm as follows
\begin{algorithm}[!hbpt]
    \caption{Score function estimation (approximate $\grad\ln p_{k,t}(\vx)$)}
    \label{alg:sfe}
    \begin{algorithmic}[1]
            \STATE {\bfseries Input:} Initial iteration number $k$ and timestamp $t$, variable $\vx$ requiring the score function;
            \IF{$k\equiv -1$ and $t\equiv 2\eta$}
                \STATE {\bfseries Return:} $-\grad f_*(\vx)$. 
            \ENDIF
            \STATE Initial the returned vector $\vv = \vzero$;
            \FOR{$i = 1$ to $n_{k,t}$}
                \STATE Draw a particle $\vx_0^\prime$ from initial distribution $q^\prime_{0}$;
                \FOR{$i = 0$ to $s_{k,t}-1$}
                    \IF{$t\equiv 2\eta$}
                        \STATE Obtain $\grad \ln p_{k,\eta}(\vx^\prime_j)$ by Alg~\ref{alg:sfe} with input $(k,\eta,\vx^\prime_j)$;
                        \STATE Update the particle with $$\vx^\prime_{j+1} = \vx^\prime_j + \tau_{k,2\eta}\cdot \left(\grad\ln p_{k,\eta}(\vx_j^\prime) + \frac{\vx -\frac{1}{2\eta c_0+1}\vx_j^\prime }{\eta}\right) + \sqrt{2\tau_{k,2\eta}}\xi$$ where $\xi$ is sampled from $\mathcal{N}(\vzero, \mI)$;
                    \ELSIF{$t\equiv \eta$}
                        \STATE Obtain $\grad\ln p_{k-1,2\eta}(\vx_j^\prime)$ by Alg~\ref{alg:sfe} with input $(k-1,2\eta,\vx_j^\prime)$;
                        \STATE Update the particle with $$\vx^\prime_{j+1} = \vx^\prime_j + \tau_{k,\eta}\cdot \left(\grad\ln p_{k-1,2\eta}(\vx_j^\prime) + \frac{\vx -\vx_j^\prime }{\eta}\right) + \sqrt{2\tau_{k,\eta}}\xi$$ where $\xi$ is sampled from $\mathcal{N}(\vzero, \mI)$;
                    \ENDIF
                \ENDFOR
                \IF{$t\equiv 2\eta$}
                    \STATE Update returned vector $\vv = \vv + \left(\eta n_{k,2\eta}\right)^{-1}\cdot \left(\vx^\prime_{s_{k,2\eta}}-(2\eta c_0+1)\vx \right)$;
                \ELSIF{$t\equiv \eta$}
                    \STATE Update returned vector $\vv = \vv + \left(\eta n_{k,2\eta}\right)^{-1}\cdot \left(\vx^\prime_{s_{k,2\eta}}-\vx \right)$;
                \ENDIF
            \ENDFOR
            \STATE {\bfseries Return:} $\vv$.
    \end{algorithmic}
\end{algorithm}

For analysis convenience, we summarize some processes as follows.
The first SDE denotes the forward process.
\begin{equation}
    \label{eq:ps_sde_forward}
    \begin{aligned}
        &\rvx_{0,0}\sim p_{0,0} = p_{*}\quad &\\
        & \der \rvx_{k,t} = \der B_t\quad &k\ge 0, t\in[0,\eta)\\
        & \der \rvx_{k,t} = -\frac{\ln(2\eta c_0+1)}{\eta} \cdot \rvx_{k,t}\der t + \sqrt{\frac{(2\eta c_0+1)\ln(2\eta c_0+1)}{2\eta c_0(\eta c_0+1)}}\der B_t\quad & k\ge 0, t\in[\eta,2\eta)\\
        &\rvx_{k+1,0}=\rvx_{k,2\eta}\quad & k\ge 0.
    \end{aligned}
\end{equation}
The second SDE denotes the ideal backward process.
\begin{equation}
    \label{eq:ps_sde_backward_ide}
    \begin{aligned}
        &\hat{\rvx}_{K,0} \sim p_{K,2\eta}\quad &\\
        &\der \hat{\rvx}_{k,t} = \left[\frac{\ln(2\eta c_0+1)}{\eta}\cdot \hat{\rvx}_{k,t} + \frac{(2\eta c_0+1)\ln(2\eta c_0+1)}{2\eta c_0 (\eta c_0+1)}\grad\ln p_{k,2\eta -t}(\hat{\rvx}_{k,t})\right]\der t\quad & \\
        &\qquad\qquad +\sqrt{\frac{(2\eta c_0+1)\ln(2\eta c_0+1)}{2\eta c_0(\eta c_0 +1)}}\der B_t\quad & k\ge 0, t\in[0,\eta)\\
        & \der \hat{\rvx}_{k,t} = \grad\ln p_{k,2\eta - t}(\hat{\rvx}_{k,t})\der t + \der B_t \quad & k\ge 0, t\in[\eta,2\eta)\\      &\hat{\rvx}_{k-1,0}=\hat{\rvx}_{k,2\eta}\quad & k\ge 1.
    \end{aligned}
\end{equation}
The third SDE denotes the practical backward process.
\begin{equation}
    \label{eq:ps_sde_backward_act}
    \begin{aligned}
        &\tilde{\rvx}_{K,0} \sim p_{K,2\eta}\quad &\\
        &\der \tilde{\rvx}_{k,t} = \left[\frac{\ln(2\eta c_0+1)}{\eta}\cdot \tilde{\rvx}_{k,t} + \frac{(2\eta c_0+1)\ln(2\eta c_0+1)}{2\eta c_0 (\eta c_0+1)}\cdot \tilde{\vv}_{k,2\eta}\right]\der t\quad & \\
        &\qquad\qquad +\sqrt{\frac{(2\eta c_0+1)\ln(2\eta c_0+1)}{2\eta c_0(\eta c_0 +1)}}\der B_t\quad & k\ge 0, t\in[0,\eta)\\
        & \der \tilde{\rvx}_{k,t} = \tilde{\vv}_{k,\eta}\der t + \der B_t \quad & k\ge 0, t\in[\eta,2\eta)\\      &\tilde{\rvx}_{k-1,0}=\tilde{\rvx}_{k,2\eta}\quad & k\ge 1.
    \end{aligned}
\end{equation}
