# Supplementary material for: Faster Sampling without Isoperimetry via Diffusion-based Monte Carlo
Source: arXiv:2401.06325 source file (2024-01-12)
Supplement: Supplementary file 3 [file 0Bimportantlemmas.tex]

\section{Important Lemmas}

\begin{lemma}
    \label{lem:station_prop_pinfty}
    For any $k\in\mathbb{N}_+$, if $p_{k,0}\propto \exp(-f_\infty)$, then we have $p_{k+1,0}=p_{k,2\eta}=p_{k,0}$.
\end{lemma}
\begin{proof}
    Suppose $p_{k,0}$ satisfies
    \begin{equation*}
        p_{k,0}(\vx) = C_{\infty}\cdot \exp\left(-f_{\infty}(\vx)\right)\quad \mathrm{where}\quad C_\infty = \int \exp(-f_\infty(\vx))\der\vx,
    \end{equation*}
    due to the update of particles shown in Eq.~\ref{eq:den_ps_stage1}, the density function of $\rvx_{k,\eta}$ is
    \begin{equation*}
        \begin{aligned}
            p_{k,\eta}(\vx) = &\left(p_{k,0}\ast \varphi_t\right)(\vx)\\
            = & C_{\infty}\int (2\pi \eta)^{-d/2}\exp\left(-f_\infty(\vy)-\frac{\left\|\vx-\vy\right\|^2}{2\eta}\right)\der\vy.
        \end{aligned}
    \end{equation*}
    Then, follows from the update of particles shown in Eq.~\ref{eq:den_ps_stage2}, the density function of $\rvx_{k,2\eta}$ is 
    \begin{equation*}
        \begin{aligned}
            p_{k,2\eta}(\vx) = & \int p_{k,\eta}(\vy)p(\rvx_{k,2\eta}=\vx|\rvx_{k,\eta}=\vy)\der \vy\\
            = & \int_{\vy \in\R^d} \left(C_\infty \int_{\vz \in \R^d} (2\pi\eta)^{-d/2}\exp\left(-f_\infty(\vz)-\frac{\left\|\vy-\vz\right\|^2}{2\eta}\right) \der\vz\right)\cdot  \frac{\exp\left(-f_\infty(\vx)-\frac{\left\|\vx-\vy\right\|^2}{2\eta}\right)}{\int_{\vz\in\R^d} \exp\left(-f_\infty(\vz)-\frac{\left\|\vz-\vy\right\|^2}{2\eta}\right) \der \vz} \der \vy\\
            = & C_\infty \exp\left(-f_\infty(\vx)\right)\cdot \int (2\pi \eta)^{-d/2}\exp\left(-\frac{\left\|\vx-\vy\right\|^2}{2\eta}\right)\der\vy = p_{k,0}(\vx).
        \end{aligned}
    \end{equation*}
    Hence, the proof is completed.
\end{proof}

\begin{lemma}
    TBC
\end{lemma}
