# Supplementary material for: Faster Sampling without Isoperimetry via Diffusion-based Monte Carlo
Source: arXiv:2401.06325 source file (2024-01-12)
Supplement: Supplementary file 4 [file 0Cmainproofs.tex]

\section{Main proofs}
