# Supplementary material for: Faster Sampling without Isoperimetry via Diffusion-based Monte Carlo
Source: arXiv:2401.06325 source file (2024-01-12)
Supplement: Supplementary file 7 [file 0GLemLips.tex]

\section{Lipschitzness of the Scores}
Via integration by parts, we obtain that
\begin{align*}
\nabla_x \ln p_{k,s}(x) = - \int \frac{x-e^{-s}x_0}{1-e^{-2s}} p_{k,0}(x_0) e^{-\frac{\|x-e^{-s}x_0\|^2}{2(1-e^{-2s})}} d x_0
= e^s \int \nabla_{x_0} p_{k,0}(x_0) e^{-\frac{\|x-e^{-s}x_0\|^2}{2(1-e^{-2s})}} d x_0.
\end{align*}
Similarly, we know that 
\begin{align*}
\nabla_x^2 \ln p_{k,s}(x) 
= -e^{2s} \int \nabla_{x_0}^2 p_{k,0}(x_0) e^{-\frac{\|x-e^{-s}x_0\|^2}{2(1-e^{-2s})}} d x_0.
\end{align*}
If we know that $\|\nabla_{x_0}^2 p_{k,0}(x_0)\|_2 \leq L \cdot p_{k,0}(x_0)$, then we can obtain the desired Lipschitz property of the score function.

Alternatively, we can have (similar to Jianfeng's paper) that
\begin{align*}
\nabla_x^2 \ln p_{k,s}(x) 
= -e^{2s} \int \left( \nabla_{x_0}^2 \ln p_{k,0}(x_0) + \nabla_{x_0} \ln p_{k,0}(x_0) \nabla_{x_0}^\top \ln p_{k,0}(x_0) \right) p_{k,0}(x_0) e^{-\frac{\|x-e^{-s}x_0\|^2}{2(1-e^{-2s})}} d x_0.
\end{align*}
In this case, we need to bound:
\[
\int \left( \nabla_{x_0} \ln p_{k,0}(x_0) \nabla_{x_0}^\top \ln p_{k,0}(x_0) \right) p_{k,0}(x_0) e^{-\frac{\|x-e^{-s}x_0\|^2}{2(1-e^{-2s})}} d x_0.
\]
We may be able to achieve that via bounding $\int \left( \nabla_{x_0} \ln p_{k,0}(x_0) \nabla_{x_0}^\top \ln p_{k,0}(x_0) \right) p_{k,0}(x_0) d x_0$ with the Lipschitz smoothness of $p_{k,0}(x_0)$.
