# Supplementary material for: Faster Sampling without Isoperimetry via Diffusion-based Monte Carlo
Source: arXiv:2401.06325 source file (2024-01-12)
Supplement: Supplementary file 8 [file 0Bimportantlemmas_backup.tex]

\newpage
\section{Proof 2}
In this proof, we will not utilize the union bound of the total variation distance as that in Lemma~\ref{lem:concen_prop}, which may help to obtain a tighter required accuracy upper bound of inner loops.
Similar to the proof in~\citep{huang2023monte}, we need to  upper bound the law of the backward path.
Hence, we have
\begin{equation}
    \label{ineq:acu_kl_err}
    \begin{aligned}
        \KL\left(\hat{\sP}_{K-1,S}\|\tilde{\sP}^{p_{K-1,S}}_{K-1, S}\right) = & \frac{1}{4}\sum_{k=0}^{K-1} \sum_{r=0}^{R-1} \E_{\hat{\sP}_{K-1, S}}\left[\int_0^\eta \left\|2\tilde{\rvv}_{k,r \eta}(\hat{\rvx}_{k,r \eta}) - 2 \grad\ln p_{k,S-(r\eta +t)}(\hat{\rvx}_{k, r\eta+t})\right\|^2 \der t\right]\\
        = & \sum_{k=0}^{K-1}\sum_{r=0}^{R-1}\int_0^{\eta}\E_{\hat{\sP}_{K-1, S}}\left[\left\|\tilde{\rvv}_{k,r\eta}(\hat{\rvx}_{k,r\eta}) - \grad\ln p_{k,S-(r\eta +t)}(\hat{\rvx}_{k,r\eta +t})\right\|^2\right] \der t\\
        \le & \underbrace{2\sum_{k=0}^{K-1}\sum_{r=0}^{R-1}\int_0^\eta \E_{\hat{\sP}_{K-1,S}}\left[\left\|\grad\ln p_{k, S-r\eta}(\hat{\rvx}_{k,r\eta})- \grad\ln p_{k,S-(r\eta +t)}(\hat{\rvx}_{k,r\eta +t})\right\|^2\right] \der t}_{\text{Term 1}}\\
        & + \underbrace{2\sum_{k=0}^{K-1}\sum_{r=0}^{R-1}\int_0^\eta \E_{\hat{\sP}_{K-1,S}}\left[\left\|\tilde{\rvv}_{k,r\eta}(\hat{\rvx}_{k,r\eta}) - \grad \ln p_{k, S-r\eta}(\hat{\rvx}_{k,r\eta})\right\|^2\right]\der t}_{\text{Term 2}}.
    \end{aligned}
\end{equation}

For any $\vx\in \R^d$, when $\hat{\rvx}_{k,r\eta}=\vx$, we consider 
    \begin{equation}
        \label{ineq:prob_recur_1}
        \begin{aligned}
            &\sP\left[\left\|\grad\ln p_{k,S-r\eta}(\vx)-\tilde{\rvv}_{k,r\eta}(\vx)\right\|^2\le 10\epsilon\right]\\
            = & \sP\left[\left\|\grad \ln p_{k,S-r\eta}(\vx)-\tilde{\rvv}_{k,r\eta}(\vx)\right\|^2\le 10\epsilon \Big| \bigcap_{i,j} \left\|\grad\ln p_{k,0}(\vx^\prime_{i,j}) -\rvv^\prime_{k,0}(\vx^\prime_{i,j})\right\|^2\le \frac{e^{-(S-r\eta)}\epsilon^2}{64}\right]\\
            & \cdot \sP\left[\bigcap_{i,j} \left\|\grad\ln p_{k,0}(\vx^\prime_{i,j}) -\rvv^\prime_{k,0}(\vx^\prime_{i,j})\right\|^2\le \frac{e^{-(S-r\eta)}\epsilon^2}{64}\right]\\
            \ge & (1-\delta)\cdot \sP\left[\bigcap_{i,j} \left\|\grad\ln p_{k,0}(\vx^\prime_{i,j}) -\rvv^\prime_{k,0}(\vx^\prime_{i,j})\right\|^2\le \frac{e^{-S}\epsilon^2}{64}\right]\\
            \ge &(1-\delta)\cdot \prod_{i=0}^{n_{k,r}(10\epsilon^2)-1} \prod_{j=0}^{m_{k,r}(10\epsilon^2)-1}\sP\left[ \left\|\grad\ln p_{k,0}(\vx^{(1)}_{i,j}) -\rvv^\prime_{k,0}(\vx^{(1)}_{i,j})\right\|^2\le \frac{\epsilon^2}{128}\right]
        \end{aligned}
    \end{equation}
    where the first inequality follows from Lemma~\ref{lem:accu_ite} and we suppose $L\ge 1/6$ without loss of generality to establish the second inequality.

    \begin{equation*}
        \begin{aligned}
            n_{k,r}(10\epsilon^2) \coloneqq &\frac{C_n}{10\epsilon^2} = \frac{16}{\epsilon^2 \eta}\cdot \max\left\{d,-2\ln\delta\right\}\\
            \ge &\frac{16}{\epsilon (1-e^{-2\eta})}\cdot \max\left\{d,-2\ln\delta\right\} \ge \frac{16}{\epsilon (1-e^{-2(S-r\eta)})} \cdot \max\left\{d, -2\ln \delta\right\}\\
            m_{k,r}(10\epsilon^2) \coloneqq & \frac{C_m}{\left(10\epsilon^2\right)^2} \coloneqq 576\cdot \frac{d}{\epsilon^2 \eta}\cdot \frac{2C_0}{\epsilon^2\eta} \ge 576\cdot\frac{d}{\epsilon^2\eta}\ln\frac{2C_0}{\epsilon^2\eta}\\
            \ge & 64\cdot \frac{L_r^2}{\mu_r^2}\cdot \frac{d}{(1-e^{-2\eta})\epsilon^2 }\ln \frac{2C_0}{(1-e^{-2\eta})\epsilon}\ge \frac{64L_r^2 d }{\mu_r^2 (1-e^{-2(S-r\eta)}) \epsilon^2}\cdot \ln \frac{2C_0}{(1-e^{-2(S-r\eta)})\epsilon^2},
        \end{aligned}
    \end{equation*}
    which implies the constants satisfy
    \begin{equation*}
        C_n = \frac{160}{\eta}\cdot \max\left\{d,-2\ln\delta\right\}\quad\text{and}\quad C_m= \frac{2^9\cdot 3^2\cdot 5^2 C_0 d}{\eta^2}.
    \end{equation*}

Eq.~\ref{ineq:prob_recur_1} shows that, for estimating the score function of each $\vx^{(0)}$ (or $\grad\ln p_{k,S-r\eta}(\vx^{(0)})$), it requires to estimate $\grad\ln p_{k,0}(\vx^{(1)})$ at least 
\begin{equation*}
    u_0\coloneqq n_{k,r}(10\epsilon^2)\cdot m_{k,r}(10\epsilon^2) = \frac{C_nC_m}{\left(10\epsilon^2\right)^3}
\end{equation*}
times if $k>0$. 
Similarly, for estimating the score function of each $\vx^{(1)}$ (or $\grad\ln p_{k,0}(\vx^{(1)})$), it requires to estimate $\grad\ln p_{k-1,0}(\vx^{(2)})$ at least 
\begin{equation*}
    u_1= n_{k-1,0}\left(\frac{\epsilon^2}{128}\right)\cdot  m_{k-1,0}\left(\frac{\epsilon^2}{128}\right) = \frac{C_nC_m}{\left(\frac{\epsilon^2}{128}\right)^3}=\frac{C_nC_m}{(10\epsilon^2)^3}\cdot 1280^3=(1280)^3 u_0
\end{equation*}
times if $k>1$. 
Due to the range of $k$ satisfying
\begin{equation*}
    k=\left\{0, 1, \ldots K-1\right\}\quad \text{where}\quad K\coloneqq \frac{T}{S} = \frac{2}{S}\ln \frac{C_I}{2\epsilon^2},
\end{equation*}
for estimating the score function of each $\vx^{(0)}$ (or $\grad\ln p_{K-1,S-r\eta}(\vx^{(0)})$), it requires to estimate $\grad\ln p_{1,0}(\vx^{(K-1)})$ at least
\begin{equation*}
    \begin{aligned}
        \prod_{i=0}^{K-2} u_i = u_0\cdot 1280^{3}u_0\cdot  \ldots \cdot 1280^{3(K-2)}u_0 = \underbrace{1280^{1.5(K-2)(K-1)}}_{\text{Term I.1}}\cdot  \underbrace{u_0^{(K-1)}}_{\text{Term I.2}}
    \end{aligned}
\end{equation*}
times. 
For Term I.1, we have
\begin{equation*}
    \begin{aligned}
        &\ln\left(\text{Term I.1}\right) = 1.5(K-2)(K-1)\ln\left(1280\right)\le 1.5\ln(1280)K^2 \le \frac{43}{S^2}\left(\ln \frac{C_I}{2\epsilon^2}\right)^2\\
        \Rightarrow & \text{Term I.1} \le \left(\frac{C_I}{2\epsilon^2}\right)^{\frac{43}{S^2}\ln \frac{C_I}{2\epsilon^2}} = \left(\frac{C_I}{2}\right)^{\frac{43}{S^2}\ln \frac{C_I}{2\epsilon^2}} \cdot \epsilon^{-\frac{86}{S^2}\ln \frac{C_I}{2\epsilon^2}}\\
        &\qquad =C_{I.1}\cdot \epsilon^{-\frac{86}{S^2}\ln\frac{C_I}{2}}\cdot \epsilon^{-\frac{86}{S^2}\ln \frac{C_I}{2\epsilon^2}}=C_{I.1}\epsilon^{-\frac{172}{S^2}\ln \frac{C_I}{2\epsilon}}\quad\text{where}\quad C_{I.1}\coloneqq \left(\frac{C_I}{2}\right)^{\frac{43}{S^2}\ln \frac{C_I}{2}}.
    \end{aligned}    
\end{equation*}

For Term I.2, we have
\begin{equation*}
    \begin{aligned}
        \ln\left(\text{Term I.2}\right) = &(K-1)\cdot \left(\ln \frac{C_nC_m}{10^3} + \ln \frac{1}{\epsilon^6}\right)\\
        \le & K\cdot \left(\ln \frac{160 \cdot \max\left\{d,2\ln\frac{1}{\delta}\right\} \cdot 2^9 \cdot 3^2\cdot 5^2 C_0d }{10^3 \eta^3} + \ln \frac{1}{\epsilon^6}\right)\\
        \le & \frac{2}{S}\ln\frac{C_I}{2\epsilon^2}\cdot \left(11+\ln C_0+ 2\ln d+\ln\ln\frac{1}{\delta} + 3\ln \frac{1}{\eta}+6\ln \frac{1}{\epsilon}\right),
    \end{aligned}
\end{equation*}
which means
\begin{equation*}
    \begin{aligned}
        \text{Term I.2} \le C_{I.2} \cdot \epsilon^{-\frac{4}{S}\left(11+\ln C_0\right)}\cdot d^{\frac{4}{S}\ln \frac{C_I}{2\epsilon^2}}\cdot (-\ln\delta)^{\frac{2}{S}\ln\frac{C_0}{2\epsilon^2}}\cdot \eta^{-\frac{6}{S}\ln \frac{C_I}{2\epsilon^2}}\cdot  \epsilon^{-\frac{12}{S}\ln \frac{C_I}{2\epsilon^2}}\\
        \text{where}\quad C_{I.2}\coloneqq \left(\frac{C_I}{2}\right)^{\frac{2}{S}\left(11+\ln C_0\right)}.
    \end{aligned}
\end{equation*}

\textcolor{blue}{--------------------------}





It means the final gradient complexity will be
\begin{equation*}
    \begin{aligned}
        \frac{T}{\eta} \cdot \text{Term I.1}\cdot \text{Term I.2} = &\frac{2}{\eta}\ln \frac{C_I}{2\epsilon^2}\cdot C_{I.1}C_{I.2}\cdot \text{Pow}\left(\epsilon, -\frac{172}{S^2}\ln \frac{C_I}{2\epsilon} -\frac{4}{S}\left(11+\ln C_0\right)-\frac{12}{S}\ln \frac{C_I}{2\epsilon^2}\right) \\
        & \cdot \text{Pow}\left(d, \frac{4}{S}\ln \frac{C_I}{2\epsilon^2}\right)\cdot \text{Pow}\left(\eta, -\frac{6}{S}\ln \frac{C_I}{2\epsilon^2}\right)\cdot \text{Pow}\left(-\ln \delta, \frac{2}{S}\ln\frac{C_0}{2\epsilon^2}\right).
    \end{aligned}
\end{equation*}

In this condition, we have
\begin{equation*}
    \begin{aligned}
        &\sP\left[\bigcap_{k,r}\left\|\grad\ln p_{k,S-r\eta}(\tilde{\vx}_{k,r\eta})-\tilde{\rvv}_{k,r\eta}(\tilde{\vx}_{k,r\eta})\right\|^2\le 10\epsilon^2\right] \ge  \text{Pow}\left(1-\delta, \frac{T}{\eta}\left(1+u_0+u_0u_1+\ldots+\prod_{i=0}^{K-2}u_i\right)\right)\\
        \ge & 1-\delta \cdot \frac{T}{\eta}\cdot K \prod_{i=0}^{K-2}u_i = 1-\delta\cdot \frac{T^2}{S\eta} \prod_{i=0}^{K-2}u_i.
    \end{aligned}
\end{equation*}
By supposing
\begin{equation*}
    \small
    \begin{aligned}
        C_B \coloneqq \frac{4}{S\eta}\left(\ln \frac{C_I}{2\epsilon^2}\right)^2\cdot C_{I.1}C_{I.2}\cdot \text{Pow}\left(\epsilon, -\frac{172}{S^2}\ln \frac{C_I}{2\epsilon} -\frac{4}{S}\left(11+\ln C_0\right)-\frac{12}{S}\ln \frac{C_I}{2\epsilon^2}\right)\cdot \text{Pow}\left(d, \frac{4}{S}\ln \frac{C_I}{2\epsilon^2}\right)\cdot \text{Pow}\left(\eta, -\frac{6}{S}\ln \frac{C_I}{2\epsilon^2}\right),
    \end{aligned}
\end{equation*}
we have $\sP\left[\bigcap_{k,r}\left\|\grad\ln p_{k,S-r\eta}(\tilde{\vx}_{k,r\eta})-\tilde{\rvv}_{k,r\eta}(\tilde{\vx}_{k,r\eta})\right\|^2\le 10\epsilon^2\right]\ge 1-\epsilon$ is equivalent to 
\begin{equation*}
    C_B\delta (-\ln \delta)^{\frac{2}{S}\ln \frac{C_I}{2\epsilon^2}}\le \epsilon\quad \Leftrightarrow\quad (-\ln \delta)^{\frac{2}{S}\ln \frac{C_I}{2\epsilon^2}}\le \frac{\epsilon}{C_B \delta} \quad \Leftrightarrow\quad \frac{2}{S}\ln \frac{C_I}{2\epsilon^2}\cdot \ln\ln\frac{1}{\delta}\le \ln \frac{\epsilon}{ C_B \delta}.
\end{equation*}
In this condition, we suppose $\delta = \epsilon/C_B \cdot \text{Pow}(a,-\frac{2}{S}\ln \frac{C_I}{2\epsilon^2})$ and have the sufficient condition can be 
\begin{equation*}
    \begin{aligned}
        &\ln \left[ \ln \frac{C_B}{\epsilon}+\frac{2}{S}\ln\frac{C_I}{2\epsilon^2}\ln a\right]\le \ln a\\
        \Leftarrow & \ln \frac{C_B}{\epsilon}\le \frac{a}{2}\quad \text{and}\quad \frac{2}{S}\ln \frac{C_I}{\epsilon}\ln a \le \frac{a}{2}\quad  \Leftarrow a\ge \frac{2C_B}{\epsilon}.
    \end{aligned}
\end{equation*}
In this condition, we have
\begin{equation*}
    \begin{aligned}
        (-\ln \delta)^{\frac{2}{S}\ln \frac{C_I}{2\epsilon^2}} = & \text{Pow}\left(\ln \frac{C_B}{\epsilon}+ \frac{2}{S}\ln\frac{C_I}{2\epsilon^2}\ln \frac{C_B}{\epsilon}, \frac{2}{S}\ln \frac{C_I}{2\epsilon^2}\right)\approx  \text{Pow}\left(\epsilon, \ln(\epsilon)\right)\cdot \text{Pow}\left(d, \left(\ln \epsilon\right)\right)\cdot \text{Pow}\left(\eta, \left(\ln \epsilon\right)\right).
    \end{aligned}
\end{equation*}
Hence, the proof is completed.




%----------------------Previous Lemmas----
\newpage
