# Supplementary material for: Faster Sampling without Isoperimetry via Diffusion-based Monte Carlo
Source: arXiv:2401.06325 source file (2024-01-12)
Supplement: Supplementary file 9 [file backup.tex]

Here, we focus on the high probability upper bound of Term 2 in Eq.~\ref{ineq:acu_kl_err}.
Hence, we have
\begin{equation*}
    \sP\left[\bigcap_{k,r} \left\|\grad \ln p_{k,S-r\eta}(\tilde{\vx}_{k,r\eta})-\tilde{\rvv}_{k,r\eta}(\tilde{\vx}_{k,r\eta})\right\|^2\le 10\epsilon^2\right] \ge  \prod^{K-1}_{k=0}\prod^{R-1}_{r=0} \sP\left[\left\|\grad \ln p_{k,S-r\eta}(\tilde{\vx}_{k,r\eta})-\tilde{\rvv}_{k,r\eta}(\tilde{\vx}_{k,r\eta})\right\|^2\le 10\epsilon^2\right].
\end{equation*}
For each pair $(k,r)$, supposing $L\ge 1/6$ without loss of generality, we have
\begin{equation}
    \label{ineq:prob_recur_1}
    \begin{aligned}
        &\sP\left[\left\|\grad \ln p_{k,S-r\eta}(\tilde{\vx}_{k,r\eta})-\tilde{\rvv}_{k,r\eta}(\tilde{\vx}_{k,r\eta})\right\|^2\le 10\epsilon^2\right]\\
        = & \sP\left[\left\|\grad \ln p_{k,S-r\eta}(\tilde{\vx}_{k,r\eta})-\tilde{\rvv}_{k,r\eta}(\tilde{\vx}_{k,r\eta})\right\|^2\le 10\epsilon^2 \Big| \bigcap_{i,j} \left\|\grad\ln p_{k,0}(\vx^\prime_{i,j}) -\rvv^\prime_{k,0}(\vx^\prime_{i,j})\right\|^2\le \frac{e^{-(S-r\eta)}\epsilon^2}{64}\right]\\
        & \cdot \sP\left[\bigcap_{i,j} \left\|\grad\ln p_{k,0}(\vx^\prime_{i,j}) -\rvv^\prime_{k,0}(\vx^\prime_{i,j})\right\|^2\le \frac{e^{-(S-r\eta)}\epsilon^2}{64}\right]\\
        \ge & (1-\delta)\cdot \sP\left[\bigcap_{i,j} \left\|\grad\ln p_{k,0}(\vx^\prime_{i,j}) -\rvv^\prime_{k,0}(\vx^\prime_{i,j})\right\|^2\le \frac{e^{-S}\epsilon^2}{64}\right]\\
        \ge &(1-\delta)\cdot \prod_{i=0}^{n_{k,r}-1} \prod_{j=0}^{m_{k,r}-1}\sP\left[ \left\|\grad\ln p_{k,0}(\vx^\prime_{i,j}) -\rvv^\prime_{k,0}(\vx^\prime_{i,j})\right\|^2\le \frac{\epsilon^2}{128}\right]
    \end{aligned}
\end{equation}
where the first inequality follows from Lemma~\ref{lem:accu_ite} by requiring
\begin{equation*}
    n_{k,r}\ge \frac{16}{\epsilon^2 (1-e^{-2(S-r\eta)})} \cdot \max\left\{d, -2\ln \delta\right\}\quad \text{and}\quad m_{k,r}\ge \frac{1}{\mu_r}\cdot \frac{64L_r^2 d }{\mu_r (1-e^{-2(S-r\eta)}) \epsilon^2}\cdot \ln \frac{2C_0}{(1-e^{-2(S-r\eta)})\epsilon^2}.
\end{equation*}
By choosing $\eta\le 1/2$, the sufficient conditions are
\begin{equation*}
    \begin{aligned}
        n_{k,r}\ge &\frac{16}{\epsilon^2 \eta}\cdot \max\left\{d,-2\ln\delta\right\}\ge \frac{16}{\epsilon^2 (1-e^{-2\eta})}\cdot \max\left\{d,-2\ln\delta\right\} \ge \frac{16}{\epsilon^2 (1-e^{-2(S-r\eta)})} \cdot \max\left\{d, -2\ln \delta\right\}\\
        m_{k,r}\ge & 576\cdot\frac{d}{\epsilon^2\eta}\ln\frac{2C_0}{\epsilon^2\eta}\ge 64\cdot \frac{L_r^2}{\mu_r^2}\cdot \frac{d}{(1-e^{-2\eta})\epsilon^2 }\ln \frac{2C_0}{(1-e^{-2\eta})\epsilon}\ge \frac{64L_r^2 d }{\mu_r^2 (1-e^{-2(S-r\eta)}) \epsilon^2}\cdot \ln \frac{2C_0}{(1-e^{-2(S-r\eta)})\epsilon^2}.
    \end{aligned}
\end{equation*}
Therefore, we have
\begin{equation*}
    \begin{aligned}
        &\sP\left[\bigcap_{k,r} \left\|\grad \ln p_{k,S-r\eta}(\tilde{\vx}_{k,r\eta})-\tilde{\rvv}_{k,r\eta}(\tilde{\vx}_{k,r\eta})\right\|^2\le 10\epsilon^2\right]\\
        \ge & (1-\delta)^{KR}\cdot \text{Pow}\left(\sP\left[ \left\|\grad\ln p_{k,0}(\vx^\prime) -\rvv^\prime_{k,0}(\vx^\prime)\right\|^2\le \frac{\epsilon^2}{128}\right], KR\cdot \frac{2^{10}\cdot 3^2 d \max\left\{d,-2\ln\delta\right\} }{\epsilon^4 \eta^2}\cdot \ln \frac{2C_0}{\epsilon^2\eta}\right)\\
        \ge & (1-\delta)^{KR}\cdot (1-\delta)^{KR\cdot \frac{2^{10}\cdot 3^2 d \max\left\{d,-2\ln\delta\right\} }{\epsilon^4 \eta^2}\cdot \ln \frac{2C_0}{\epsilon^2\eta}}\\
    \end{aligned}
\end{equation*}


\section{Proof 1}

Similar to the proof in~\citep{huang2023monte}, we need to  upper bound the law of the backward path.
Hence, we have
\begin{equation*}
    \begin{aligned}
        \KL\left(\hat{\sP}_{K-1,S}\|\tilde{\sP}^{p_{K-1,S}}_{K-1, S}\right) = & \frac{1}{4}\sum_{k=0}^{K-1} \sum_{r=0}^{R-1} \E_{\hat{\sP}_{K-1, S}}\left[\int_0^\eta \left\|2\tilde{\rvv}_{k,r \eta}(\hat{\rvx}_{k,r \eta}) - 2 \grad\ln p_{k,S-(r\eta +t)}(\hat{\rvx}_{k, r\eta+t})\right\|^2 \der t\right]\\
        = & \sum_{k=0}^{K-1}\sum_{r=0}^{R-1}\int_0^{\eta}\E_{\hat{\sP}_{K-1, S}}\left[\left\|\tilde{\rvv}_{k,r\eta}(\hat{\rvx}_{k,r\eta}) - \grad\ln p_{k,S-(r\eta +t)}(\hat{\rvx}_{k,r\eta +t})\right\|^2\right] \der t\\
        \le & \underbrace{2\sum_{k=0}^{K-1}\sum_{r=0}^{R-1}\int_0^\eta \E_{\hat{\sP}_{K-1,S}}\left[\left\|\grad\ln p_{k, S-r\eta}(\hat{\rvx}_{k,r\eta})- \grad\ln p_{k,S-(r\eta +t)}(\hat{\rvx}_{k,r\eta +t})\right\|^2\right] \der t}_{\text{Term 1}}\\
        & + \underbrace{2\sum_{k=0}^{K-1}\sum_{r=0}^{R-1}\int_0^\eta \E_{\hat{\sP}_{K-1,S}}\left[\left\|\tilde{\rvv}_{k,r\eta}(\hat{\rvx}_{k,r\eta}) - \grad \ln p_{k, S-r\eta}(\hat{\rvx}_{k,r\eta})\right\|^2\right]\der t}_{\text{Term 2}}
    \end{aligned}
\end{equation*}
In the upper bound, Term 1 shares the same upper bound as that in~\citep{huang2023monte}.
Here, we focus on the upper bound of Term 2.
According to the Algorithm~\ref{alg:bpsa}, suppose the underlying distribution of $\vx^\prime_{i,m_{k,r}}$ is $\tilde{q}_{k, S-r\eta}(\cdot |\tilde{\vx}_{k,S-r\eta})$ which can be considered as the approximation of the following distribution 
\begin{equation}
    \label{ineq:aux_q_def}
    q_{k,S-r\eta}(\vx^\prime | \vx)\propto p_{k,0}(\vx^\prime)\cdot \exp\left[-\frac{\left\|\vx-e^{-(S-r\eta)}\vx^\prime\right\|^2}{2(1-e^{-2(S-r\eta)})}\right].
\end{equation}

\begin{lemma}
    \label{lem:concen_prop}
    In Alg~\ref{alg:bpsa}, for any $\vx\in \R^d$, when $\hat{\rvx}_{k,r\eta}=\vx$, we have
    \begin{equation*}
        \sP\left[\left\|\tilde{\rvv}_{k,r\eta}(\vx) - \grad\ln p_{k,S-r\eta}(\vx)\right\|\le 2\epsilon \right] \ge 1-2\delta
    \end{equation*}
    by requiring the sample number $n_k$ and the underlying distribution of $\vx^\prime_{i,m_{k,r}}$, i.e., $\tilde{q}_{k,S-r\eta}(\cdot|\vx)$ satisfy
    \begin{equation*}
        n_k \ge L^{-1}\epsilon^{-2}\eta^{-2}\cdot \max\left\{d, -\ln\delta\right\}\quad\text{and}\quad \TVD(q_{k,S-r\eta}(\cdot|\vx), \tilde{q}_{k,S-r\eta}(\cdot|\vx)) \le \delta/n_k.
    \end{equation*}
\end{lemma}
\begin{proof}
    In this lemma, we mainly analyze the sample number required for each iteration of Alg~\ref{alg:bpsa} when the $\vv_j^\prime$ is given.
    Hence, it is suitable for any specific $r$ and $k$.
    To simplify the notation, we abbreviate $\vx^\prime_{i, m_{k,r}}$ as $\vx^\prime_i$.

    
    For any $\vx\in \R^d$, when $\hat{\rvx}_{k,r\eta}=\vx$, we
    set
    \begin{equation*}
        \begin{aligned}
            & \tilde{\vb} \coloneqq \E_{\tilde{q}_{k,S-r\eta}(\cdot|\vx)}\left[\rvx^\prime\right]\quad && \tilde{\sigma}\coloneqq \E_{\left\{\rvx^\prime_i\right\}_{i=0}^{n_k-1}\sim \tilde{q}^{(n_k)}_{k,S-r\eta}(\cdot|\vx)  }\left[\left\|\sum_{i=0}^{n_k-1}\rvx_i - \E\left[\sum_{i=0}^{n_k-1}\rvx_i\right]\right\|\right]\\
            & \vb \coloneqq \E_{q_{k,S-r\eta}(\cdot|\vx)}\left[\rvx^\prime\right] && \sigma\coloneqq \E_{\left\{\rvx^\prime_i\right\}_{i=0}^{n_k-1}\sim q^{(n_k)}_{k,S-r\eta}(\cdot|\vx)  }\left[\left\|\sum_{i=0}^{n_k-1}\rvx_i - \E\left[\sum_{i=0}^{n_k-1}\rvx_i\right]\right\|\right].
        \end{aligned}
    \end{equation*}
    
    
    Then, considering the following probability
    \begin{equation}
        \label{ineq:upb_concen_sp}
        \small
        \begin{aligned}
            &\sP\left[\left\|\tilde{\rvv}_{k,r\eta}(\vx) - \grad\ln p_{k,S-r\eta}(\vx)\right\|\ge \frac{e^{-(S-r\eta)}}{1-e^{-2(S-r\eta)}}\cdot \frac{\sigma}{n_k} +\epsilon \right] \\
            = &\sP_{\left\{\rvx_i^\prime\right\}_{i=0}^{n_k-1} \sim \tilde{q}^{(n_k)}_{k,S-r\eta}(\cdot|\vx) }\left[\left\|\frac{1}{n_k}\sum_{i=0}^{n_k-1}\left(-\frac{\vx - e^{-(S-r\eta)}\rvx_i^\prime}{1-e^{-2(S-r\eta)}}\right)-\E_{\rvx^\prime\sim q_{k,S-r\eta}(\cdot|\vx)}\left[-\frac{\vx - e^{-(S-r\eta)}\rvx^\prime }{1-e^{-2(S-r\eta)}}\right] \right\|\ge \frac{e^{-(S-r\eta)}}{1-e^{-2(S-r\eta)}}\cdot \frac{\sigma}{n_k} +\epsilon\right]\\
            = & \sP_{\left\{\rvx_i^\prime\right\}_{i=0}^{n_k-1} \sim \tilde{q}^{(n_k)}_{k,S-r\eta}(\cdot|\vx) }\left[\left\|\sum_{i=0}^{n_k-1} \rvx_i^\prime- n_k\vb \right\|\ge \sigma + \frac{n_k (1-e^{-2(S-r\eta)})}{e^{-(S-r\eta)}}\cdot \epsilon\right]\\
            \le & \sP_{\left\{\rvx_i^\prime\right\}_{i=0}^{n_k-1} \sim q^{(n_k)}_{k,S-r\eta}(\cdot|\vx) }\left[\left\|\sum_{i=0}^{n_k-1} \rvx_i^\prime- n_k\vb \right\|\ge \sigma + \frac{n_k (1-e^{-2(S-r\eta)})}{e^{-(S-r\eta)}}\cdot \epsilon\right]  + \TVD(q^{(n_k)}_{k,S-r\eta}(\cdot|\vx), \tilde{q}^{(n_k)}_{k,S-r\eta}(\cdot|\vx))\\
            \le & \underbrace{\sP_{\left\{\rvx_i^\prime\right\}_{i=0}^{n_k-1} \sim q^{(n_k)}_{k,S-r\eta}(\cdot|\vx) }\left[\left\|\sum_{i=0}^{n_k-1} \rvx_i^\prime- n_k\vb \right\|\ge \sigma + \frac{n_k (1-e^{-2(S-r\eta)})}{e^{-(S-r\eta)}}\cdot \epsilon\right]}_{\text{Term 1}} + n_k \cdot \underbrace{\TVD(q_{k,S-r\eta}(\cdot|\vx), \tilde{q}_{k,S-r\eta}(\cdot|\vx))}_{\text{Term 2}}.
        \end{aligned}
    \end{equation}

    \paragraph{Upper bound Term 1:}According to Eq.~\ref{ineq:aux_q_def}, i.e., the formulation of $q_{k,S-r\eta}(\cdot|\vx)$, we have 
    \begin{equation*}
        L\mI \preceq \grad^2 \ln q_{k,S-r\eta}(\cdot|\vx)  \preceq 3L,
    \end{equation*}
    which means $q_{k,S-r\eta}(\cdot|\vx)$ satisfies LSI with constant $L$ due to Lemma~\ref{lem:strongly_lsi}.
    Besides, Lemma~\ref{lem_conv} implies the LSI constant of
    \begin{equation*}
        \sum_{i=1}^{n}\rvx_i^\prime \sim \underbrace{q_{k,S-r\eta}(\cdot|\vx) \ast q_{k,S-r\eta}(\cdot|\vx) \cdots \ast q_{k,S-r\eta}(\cdot|\vx)}_{n_k}
    \end{equation*}
    is  $L/n_k$. 
    Considering the function $F\left( \vx \right) = \left\| \vx \right\| \colon \R^{d}\rightarrow \R$ is $1$-Lipschitz because
    \begin{equation*}
        \left\|F\right\|_{\mathrm{Lip}}=\sup_{\vx \not= \vy} \frac{\left|F(\vx)-F(\vy)\right|}{\left\|\vx - \vy\right\|}=\sup_{\vx\not = \vy}\frac{\left|\left\| \vx \right\| - \left\| \vy \right\|\right|}{\left\| \left(\vx - \vy \right)\right\|} = 1,
    \end{equation*}
    we have 
    \begin{equation}
        \label{ineq:upb_concen_term1}
        \small
        \sP_{\left\{\rvx_i^\prime\right\}_{i=0}^{n_k-1} \sim q^{(n_k)}_{k,S-r\eta}(\cdot|\vx) }\left[\left\|\sum_{i=0}^{n_k-1} \rvx_i^\prime- n_k\vb \right\|\ge \sigma + \frac{n_k (1-e^{-2(S-r\eta)})}{e^{-(S-r\eta)}}\cdot \epsilon\right]\le \exp\left(-\frac{Ln_k\epsilon^2(1-e^{-(S-2r\eta)})^2}{2e^{-2(S-r\eta)}}\right).
    \end{equation}

    \paragraph{Upper bound Term 2:} Actually, the upper bound of Term 2 depends on the accuracy required in ULA (Line. 8 -- Line. 11 in Alg~\ref{alg:bpsa}).
    Here, we require 
    \begin{equation}
        \label{ineq:upb_concen_term2}
        \TVD(q_{k,S-r\eta}(\cdot|\vx), \tilde{q}_{k,S-r\eta}(\cdot|\vx)) \le \delta/n_k.
    \end{equation}

    Combining Eq.~\ref{ineq:upb_concen_sp}, Eq.~\ref{ineq:upb_concen_term1} and Eq.~\ref{ineq:upb_concen_term2}, we have
    \begin{equation*}
        \begin{aligned}
            &\sP\left[\left\|\tilde{\rvv}_{k,r\eta}(\vx) - \grad\ln p_{k,S-r\eta}(\vx)\right\|\ge \frac{e^{-(S-r\eta)}}{1-e^{-2(S-r\eta)}}\cdot \frac{\sigma}{n_k} +\epsilon \right] \le \exp\left(-\frac{Ln_k\epsilon^2(1-e^{-(S-2r\eta)})^2}{2e^{-2(S-r\eta)}}\right) + \delta.
        \end{aligned}
    \end{equation*}
    Besides, we can upper bound $\sigma$ with Lemma~\ref{lem:lsi_var_bound} and have
    \begin{equation*}
        \begin{aligned}
            \sigma = n_k\cdot \mathbb{E}_{\left\{\rvx_i^\prime\right\}_{i=0}^{n_k-1} \sim q^{(n_k)}_{k,S-r\eta}(\cdot|\vx)}\left\| \frac{1}{n_k}\sum_{i=0}^{n_k-1} \rvx_i^\prime - \vb\right\| \le n_k\cdot \sqrt{\mathrm{var}\left(\frac{1}{n_k}\sum_{i=1}^{n_k} \rvx_i^\prime\right)}= \sqrt{n_k \mathrm{var}\left(\rvx_i^\prime\right)} \le \sqrt{\frac{n_k d}{L}}.
        \end{aligned}
    \end{equation*}
    Hence, we have
    \begin{equation*}
        \begin{aligned}
            &\sP\left[\left\|\tilde{\rvv}_{k,r\eta}(\vx) - \grad\ln p_{k,S-r\eta}(\vx)\right\|\ge \frac{e^{-(S-r\eta)}}{1-e^{-2(S-r\eta)}}\cdot \sqrt{\frac{d}{Ln_k}} +\epsilon \right]\le \exp\left(-\frac{Ln_k\epsilon^2(1-e^{-(S-2r\eta)})^2}{2e^{-2(S-r\eta)}}\right) + \delta.
        \end{aligned}
    \end{equation*}
    By requiring 
    \begin{equation}
        \label{ineq:sample_req}
        \frac{e^{-(S-r\eta)}}{1-e^{-2(S-r\eta)}}\cdot \sqrt{\frac{d}{Ln_k}}\le \epsilon \quad\text{and}\quad -\frac{Ln_k\epsilon^2(1-e^{-(S-2r\eta)})^2}{2e^{-2(S-r\eta)}}\le \ln\delta,
    \end{equation}
    we have
    \begin{equation*}
        \begin{aligned}
            \sP\left[\left\|\tilde{\rvv}_{k,r\eta}(\vx) - \grad\ln p_{k,S-r\eta}(\vx)\right\|\le 2\epsilon \right]=  1- \sP\left[\left\|\tilde{\rvv}_{k,r\eta}(\vx) - \grad\ln p_{k,S-r\eta}(\vx)\right\|\ge 2\epsilon \right] \ge 1- 2\delta.
        \end{aligned}
    \end{equation*}
    The first inequality in Eq.~\ref{ineq:sample_req} implies the sample number $n_k$ should satisfy
    \begin{equation*}
        \begin{aligned}
            n_k \ge \frac{d}{L\epsilon^2\eta^2}\quad \Rightarrow\quad  n_k \ge \frac{d}{L\epsilon^2}\cdot \frac{e^{-2(S-r\eta)}}{(1-e^{-2(S-r\eta)})^2}\quad \Leftrightarrow\quad \frac{e^{-(S-r\eta)}}{1-e^{-2(S-r\eta)}}\cdot \sqrt{\frac{d}{Ln_k}}\le \epsilon
        \end{aligned}
    \end{equation*}
    where the second inequality establishes because we suppose $\eta\le 1/2$ without loss of generality and it has
    \begin{equation*}
        e^{-2(S-r\eta)}\le e^{-2\eta} \le 1-\eta\quad\Rightarrow \frac{e^{-2(S-r\eta)}}{(1-e^{-2(S-r\eta)})^2}\le \eta^{-2}.
    \end{equation*}
    The second inequality in Eq.~\ref{ineq:sample_req} implies
    \begin{equation*}
        n_k \ge \frac{1}{L\epsilon^2 \eta^2}\cdot \ln \frac{1}{\delta}\quad \Rightarrow\quad n_k\ge \frac{1}{L\epsilon^2}\cdot \frac{e^{-2(S-r\eta)}}{(1-e^{-2(S-r\eta)})^2}\cdot \ln \frac{1}{\delta} \quad \Leftrightarrow -\frac{Ln_k\epsilon^2(1-e^{-(S-2r\eta)})^2}{2e^{-2(S-r\eta)}}\le \ln\delta. 
    \end{equation*}
    Hence, the proof is completed.
\end{proof}

Actually, in Lemma~\ref{lem:concen_prop}, we mainly determine the range of $n_k$.
To calculate the practical computational complexity, we also need to upper bound $m_k$, which utilizes similar techniques in~\citep{vempala2019rapid}.

\begin{lemma}
    \label{lem:inner_err_conv}
    For any given $(k,r)$ in Alg~\ref{alg:bpsa}, suppose the distribution $q_{k,S-r\eta}(\cdot|\tilde{\vx}_{k,r\eta})$ satisfies
    \begin{equation*}
        \mu_r\mI \preceq -\grad^2\ln q_{k,S-r\eta}(\cdot|\tilde{\vx}_{k,r\eta}) \preceq L_r\mI,
    \end{equation*}
    and $\rvx_{i,j}^\prime \sim q_j^\prime(\cdot |\tilde{\vx}_{k,r\eta})$.
    If $0<\tau_r \le \mu_r/(4L^2_r)$, we have
    \begin{equation*}
        \KL\left(q_{j+1}^\prime\|q_*\right)\le e^{-\frac{\mu_r \tau_r}{2}}\KL\left(q_j^\prime\|q_*\right)  + 10L_r^2 d\tau_r^2
    \end{equation*}
    when the score estimation satisfies $\left\|\grad\ln p_{k,0} -\vv^\prime\right\|\le L_r\sqrt{2d\tau_r}$.
\end{lemma}
\begin{proof}
    We know that the loop in Line 8 of Alg~\ref{alg:bpsa} aims to draw a sample from the target distribution $q_{k,S-r\eta}(\cdot|\tilde{\vx}_{k,r\eta})$ abbreviated as $q_*\propto \exp(-g_*)$. 
    %Meanwhile, the maximal and minimal eigenvalue of the Hessian of negative log density ($\grad^2 g_*$), i.e., $L_r$ and $\mu_r$, are abbreviated as $L$ and $\mu$ respectively. 
    Besides, we analyze the dynamics of KL divergence in the $j$-th iteration in the loop (Line 10).
    For notation simplicity, we denote $\vv_j^\prime$ and $\tau_r$ as $\vv^\prime$ and $\tau$, and set
    \begin{equation*}
        -\grad g^\prime(\vz)=\vv^\prime + \frac{e^{-(S-r\eta)}\tilde{\vx}_{k,r\eta} - e^{-2(S-r\eta)}\vz}{1-e^{-2(S-r\eta)}} 
    \end{equation*}
    Suppose $\rvx^\prime_{i,j}=\vz_0$, the $j$-th iteration is equivalent to the following SDE
    \begin{equation*}
    \begin{aligned}
        &\der \rvz_t = -\grad g^\prime(\vz_0)\der t + \sqrt{2}\der B_t,
    \end{aligned}
    \end{equation*}
    we denote the underlying distribution of $\rvz_t$ as $q_t$.
    Similarly, we set $q_{0t}$ as the joint distribution of $(\rvz_0, \rvz_t)$, and have
    \begin{equation*}
        q_{0t}(\vz_0,\vz_t) = q_0(\vz_0)\cdot q_{t|0}(\vz_t|\vz_0).
    \end{equation*}
    According to the Fokker-Planck equation, we have
    \begin{equation*}
        \partial_t q_{t|0}(\vz_t|\vz_0)= \grad\cdot\left(q_{t|0}(\vz_t|\vz_0)\cdot \grad g^\prime(\vz_0)\right) + \Delta q_{t|0}(\vz_t|\vz_0)
    \end{equation*}
    In this condition, we have
    \begin{equation*}
        \begin{aligned}
            \partial_t q_{t}(\vx_t) = &\int \frac{\partial q_{t|0}(\vz_t|\vz_0)}{\partial t} \cdot q_0(\vz_0)\der\vz_0\\
            = & \int \left[\grad \cdot \left(q_{t|0}(\vz_t|\vz_0)\cdot \grad g^\prime(\vz_0)\right) +\Delta q_{t|0}(\vz_t|\vz_0)\right]\cdot q_0(\vz_0)\der\vz_0\\
            = & \grad\cdot \left(q_t(\vz_t)\int q_{0|t}(\vz_0|\vz_t) \grad g^\prime(\vz_0)\der\vz_0\right)+ \Delta q_t(\vz_t).
        \end{aligned}
    \end{equation*}
    Hence, the dynamics of the KL functional will be 
    \begin{equation*}
        \begin{aligned}
            \partial_t\KL\left(q_t\|q_*\right) = &\int \partial_t q_t(\vz_t)\ln \frac{q_t(\vz_t)}{q_*(\vz_t)}\der\vz_t\\
            = & \int \grad\cdot \left[q_t(\vz_t)\left(\int q_{0|t}(\vz_0|\vz_t)\grad g^\prime(\vz_0)\der\vz_0 + \grad\ln q_t(\vz_t)\right)\right]\cdot \ln \frac{q_t(\vz_t)}{q_*(\vz_t)}\der\vz_t\\
            = & -\int q_t(\vz_t)\left(\left\|\grad\ln \frac{q_t(\vz_t)}{q_*(\vz_t)}\right\|^2+\left<\int q_{0|t}(\vz_0|\vz_t)\grad g^\prime(\vz_0)\der\vz_0+\grad\ln q_*(\vz_t),\grad\ln\frac{q_t(\vz_t)}{q_*(\vz_t)}\right>\right) \der\vz_t\\
            = & -\int q_t(\vz_t)\left\|\grad \ln \frac{q_t(\vz_t)}{q_*(\vz_t)}\right\|^2 \der\vz_t\\
            & + \int q_{0t}(\vz_0, \vz_t)\left<\grad g^\prime(\vz_0)-\grad g_*(\vz_t),\grad \ln \frac{q_t(\vz_t)}{q_*(\vz_t)}\right>\der (\vz_0, \vz_t)\\
            \le & -\frac{3}{4}\int q_t(\vz_t)\left\|\grad\ln \frac{q_t(\vz_t)}{q_*(\vz_t)}\right\|^2 \der \vz_t + \int q_{0t}(\vz_0,\vz_t)\left\|\grad g^\prime(\vz_0) - \grad g_*(\vz_t)\right\|^2 \der (\vz_0,\vz_t)\\
            \le & \underbrace{-\frac{3}{4}\int q_t(\vz_t)\left\|\grad\ln \frac{q_t(\vz_t)}{q_*(\vz_t)}\right\|^2}_{\text{Term 1}} + 2\underbrace{\int q_{0t}(\vz_0,\vz_t)\left\|\grad g^\prime(\vz_0) - \grad g_*(\vz_0)\right\|^2 \der (\vz_0,\vz_t)}_{\text{Term 2}}\\
            & + 2\underbrace{\int q_{0t}(\vz_0,\vz_t)\left\|\grad g_*(\vz_0) - \grad g_*(\vz_t)\right\|^2 \der (\vz_0,\vz_t)}_{\text{Term 3}}.
        \end{aligned}
    \end{equation*}
    \paragraph{Upper bound Term 1:} The target distribution $q_*$ satisfies
    \begin{equation*}
        -\grad^2 \ln(q_*(\vx)) = -\grad^2 \ln q_{k, S-r\eta}(\vx|\tilde{\vx}_{k,r\eta})= -\grad^2\ln p_{k,0}(\vx) + \frac{e^{-2(S-r\eta)}}{1-e^{-2(S-r\eta)}} \succeq L\mI,
    \end{equation*}
    which implies the strong log-concavity of $q_*$.
    Besides, we set the $-\grad^2 \ln(q_*(\vx))\succeq \mu_r \mI$ where $\mu_q$ denotes the minimum eigenvalue of $-\grad^2 \ln(q_*(\vx))$.
    It means $q_*$ satisfies LSI with the constant $\mu_r$ due to Lemma~\ref{lem:strongly_lsi}.
    Hence, we have
    \begin{equation*}
        \text{Term 1}\le -\frac{3\mu_q}{2}\KL\left(q_t\|q_*\right).
    \end{equation*}
    \paragraph{Upper bound Term 2:} We assume that there is a uniform upper bound $\delta_g$ satisfying 
    \begin{equation*}
        \left\|\grad g^\prime(\vz)-\grad g_*(\vz)\right\| \le \delta_g\quad \Rightarrow\quad \text{Term 2}\le \delta_g^2.
    \end{equation*}
    \paragraph{Upper bound Term 3:} The target distribution $q_*$ satisfies
    \begin{equation*}
        -\grad^2 \ln(q_*(\vx)) = -\grad^2 \ln q_{k, S-r\eta}(\vx|\tilde{\vx}_{k,r\eta})= -\grad^2\ln p_{k,0}(\vx) + \frac{e^{-2(S-r\eta)}}{1-e^{-2(S-r\eta)}} \preceq (L+ \eta^{-1})\mI,
    \end{equation*}
    which implies the smoothness of $q_*$.
    Besides, we set the $-\grad^2 \ln(q_*(\vx))\preceq L_r \mI$ where $L_q$ denotes the maximal eigenvalue of $-\grad^2 \ln(q_*(\vx))$.
    In this condition, we have
    \begin{equation*}
        \begin{aligned}
            \text{Term 3}\le & L_r^2 \int q_{0t}(\vz_0, \vz_t)\left\|\vz_t - \vz_0\right\|^2 \der (\vz_0,\vz_t)= L_r^2 \cdot \E_{q_{0t}}\left[\left\|-t \grad g^\prime(\vz_0)+\sqrt{2t}\xi\right\|^2\right]\\
            = & L^2_r\cdot \left(2td +t^2\E_{q_{0}}\left\|\grad g^\prime(\vz_0)-\grad g_*(\vz_0)+\grad g_*(\vz_0)\right\|^2\right) \\
            \le & 2L_r^2 \cdot \left(td + t^2\delta_g^2 + t^2\E_{q_0}\left\|\grad g_*(\vz_0)\right\|^2\right)\\
            \le & 2L_r^2 dt +2L_r^2\delta_g^2 t^2+4L_r^3 dt^2 + \frac{8L_r^4 t^2}{\mu_r}\KL\left(q_0\|q_*\right),
        \end{aligned}
    \end{equation*}
    where the last inequality follows from Lemma~\ref{lem:rapidlem12}.
    Hence, by requiring $t\le \tau \le 1/(2L_g)$ and $\delta^2_g \le 2L_q^2 d\tau$, we have
    \begin{equation*}
        \begin{aligned}
            \partial_t\KL\left(q_t\|q_*\right) \le & -\frac{3\mu_r}{2}\KL\left(q_t\|q_*\right) +  \frac{8L_r^4 t^2}{\mu_r}\KL\left(q_0\|q_*\right) + 4L_q^4 d\tau t^2 + 4L_r^3dt^2 + 2L_r^2 dt\\
            \le &  -\frac{3\mu_r}{2}\KL\left(q_t\|q_*\right) +  \frac{8L_r^4 \tau^2}{\mu_r}\KL\left(q_0\|q_*\right) + 5L_r^2 d\tau.
        \end{aligned}
    \end{equation*}
    Multiplying both sides by $\exp(\frac{3\mu_r t}{2})$, then the previous inequality can be written as
    \begin{equation*}
        \frac{\der}{\der t}\left(e^{\frac{3\mu_r t}{2}}\KL\left(q_t\|q_*\right)\right)\le e^{\frac{3\mu_r t}{2}}\cdot \left(\frac{8L_r^4 \tau^2}{\mu_q}\KL\left(q_0\|q_*\right) + 5L_r^2 d\tau\right).
    \end{equation*}
    Integrating from $t=0$ to $t=\tau$, we have
    \begin{equation*}
        \begin{aligned}
            e^{\frac{3\mu_r \tau}{2}}\KL\left(q_t\|q_*\right) - \KL\left(q_0\|q_*\right)\le & \frac{2}{3\mu_r}\cdot \left(e^{\frac{3\mu_r \tau}{2}}-1\right)\cdot \left(\frac{8L_r^4 \tau^2}{\mu_r}\KL\left(q_0\|q_*\right) + 5L_r^2 d\tau\right)\\
            \le & 2\tau\cdot \left(\frac{8L_r^4 \tau^2}{\mu_r}\KL\left(q_0\|q_*\right) + 5L_r^2 d\tau\right)
        \end{aligned}
    \end{equation*}
    where the last inequality establishes due to the fact $e^c \le 1+2c$ when $0<c\le \frac{3}{2}\cdot \mu_q \tau\le 1$. 
    It means we have
    \begin{equation*}
        \begin{aligned}
            \KL\left(q_t\|q_*\right)\le e^{-\frac{3\mu_q \tau}{2}}\cdot \left(1+\frac{16 L_q^4 \tau^3}{\mu_q}\right)\KL\left(q_0\|q_*\right) + e^{-\frac{3\mu_q \tau}{2}}\cdot 10L_q^2 d\tau^2.
        \end{aligned}
    \end{equation*}
    By requiring $\tau\le \mu_r/(4L_r^2)$, we have 
    \begin{equation*}
        1+\frac{16 L_r^4 \tau^3}{\mu_r} \le 1+\mu_r \tau \le e^{\mu_r \tau}\quad \text{and}\quad e^{-\frac{3\mu_r \tau}{2}}\le 1.
    \end{equation*}
    Hence, there is
    \begin{equation}
        \label{ineq:suff_des_ld}
        \KL\left(q_t\|q_*\right)\le e^{-\frac{\mu_r \tau}{2}}\KL\left(q_0\|q_*\right)  + 10L_r^2 d\tau^2,
    \end{equation}
    and the proof is completed.
\end{proof}

\begin{corollary}
    \label{cor:kl_conv_inexact_grad}
    For any given $(k,r)$ in Alg~\ref{alg:bpsa}, suppose the distribution $q_{k,S-r\eta}(\cdot|\tilde{\vx}_{k,r\eta})$ satisfies
    \begin{equation*}
        \mu_r\mI \preceq -\grad^2\ln q_{k,S-r\eta}(\cdot|\tilde{\vx}_{k,r\eta}) \preceq L_r\mI,
    \end{equation*}
    and $\rvx_{i,j}^\prime \sim q_j^\prime(\cdot |\tilde{\vx}_{k,r\eta})$.
    If $0<\tau_r \le \mu_r/(4L^2_r)$, we have
    \begin{equation*}
        \exp\left(-\frac{\mu_r k\tau}{2}\right)\cdot \KL\left(q_0\|q_*\right) + \frac{24L_r^2 d\tau}{\mu_r}
    \end{equation*}
    when the score estimation satisfies $\left\|\grad\ln p_{k,0} -\vv^\prime\right\|\le L_r\sqrt{2d\tau_r}$.
\end{corollary}
\begin{proof}
    Due to the range $0<\tau\le \mu_r/4L_r^2$, we have $(\mu_r \tau)/2\le 1/8$.
    In this condition, we have 
    \begin{equation*}
        1-\exp\left(-\frac{\mu_r\tau}{2}\right)\ge \frac{5}{6}\cdot \frac{\mu_r \tau}{2} = \frac{5\mu_r \tau}{12}.
    \end{equation*}
    Plugging this into the following inequality obtained by the recursion of Eq.~\ref{ineq:suff_des_ld}, we have
    \begin{equation*}
        \begin{aligned}
            \KL\left(q_j\|q_*\right)\le &\exp\left(-\frac{\mu_r j\tau}{2}\right)\cdot \KL\left(q_0\|q_*\right) + \frac{10L_r^2 d\tau^2}{\left(1-\exp\left(-\frac{-\mu_r \tau}{2}\right)\right)}\\
            \le & \exp\left(-\frac{\mu_r j\tau}{2}\right)\cdot \KL\left(q_0\|q_*\right) + \frac{24L_r^2 d\tau}{\mu_r}.
        \end{aligned}
    \end{equation*}
    In this condition, if we require the KL divergence to satisfy $\KL\left(q_j\|q_*\right)\le \epsilon$, a sufficient condition is that 
    \begin{equation*}
        \exp\left(-\frac{\mu_r j\tau}{2}\right)\cdot \KL\left(q_0\|q_*\right)\le \frac{\epsilon}{2} \quad\text{and}\quad  24L_r^2 d\tau\le \frac{\epsilon}{2},
    \end{equation*}
    which is equivalent to 
    \begin{equation*}
        \tau\le \frac{\mu_r\epsilon}{48 L_r^2 d} \quad \text{and}\quad m_k\ge \frac{2}{\mu_r \tau}\cdot \ln\frac{2C_0}{\epsilon}.
    \end{equation*}
\end{proof}


After upper bounding the sample number and iteration complexity for each pair $(k,r)$, we are able to provide the computational complexity for a high probability convergence of the total variation distance.
\begin{equation*}
    \begin{aligned}
        &\sP\left[\bigcap_{k,r} \left\|\grad \ln p_{k,S-r\eta}(\tilde{\vx}_{k,r\eta})-\tilde{\vv}_{k,r\eta}\right\|^2\le 4\epsilon^2\right] \ge  \left(\sP\left[\left\|\grad \ln p_{k,S-r\eta}(\tilde{\vx}_{k,r\eta})-\tilde{\vv}_{k,r\eta}\right\|\le 2\epsilon\right]\right)^{\frac{T}{\eta}}\\
        = & \left(\underbrace{\sP\left[\left\|\grad \ln p_{k,S-r\eta}(\tilde{\vx}_{k,r\eta})-\tilde{\vv}_{k,r\eta}\right\|\le 2\epsilon \Big| \bigcap_{i=0}^{n_k-1}\TVD\left(\tilde{q}^{(i)}_{k,S-r\eta}(\cdot |\tilde{\vx}_{k,r\eta}),q_{k,S-r\eta}(\cdot |\tilde{\vx}_{k,r\eta})\right)\le \frac{\delta_0}{n_k}\right]}_{\text{Lemma~B.1}}\right)^{\frac{T}{\eta}}\\
        & \cdot \left(\sP \left[\bigcap_{i=1}^{n_k}\TVD\left(\tilde{q}^{(i)}_{k,S-r\eta}(\cdot |\tilde{\vx}_{k,r\eta}),q_{k,S-r\eta}(\cdot |\tilde{\vx}_{k,r\eta})\right)\le \frac{\delta_0}{n_k}\right]\right)^{\frac{T}{\eta}}\\
        \ge & (1-2\delta_0)^{\frac{T}{\eta}}\cdot \left(\sP\left[\TVD\left(\tilde{q}^{(i)}_{k,S-r\eta}(\cdot |\tilde{\vx}_{k,r\eta}),q_{k,S-r\eta}(\cdot |\tilde{\vx}_{k,r\eta})\right) \le \frac{\delta_0}{n_k}\right]\right)^{\frac{T}{\eta}\cdot n_k}\\
        \ge &  (1-2\delta_0)^{\frac{T}{\eta}}\cdot \left(\sP\left[\KL\left(\tilde{q}^{(i)}_{k,S-r\eta}(\cdot |\tilde{\vx}_{k,r\eta}),q_{k,S-r\eta}(\cdot |\tilde{\vx}_{k,r\eta})\right) \le \frac{2\delta^2_0}{n^2_k}\right]\right)^{\frac{T}{\eta}\cdot n_k} \\
        = & (1-2\delta_0)^{\frac{T}{\eta}}\cdot \left(\underbrace{\sP\left[\KL\left(\tilde{q}_{k,S-r\eta}(\cdot |\tilde{\vx}_{k,r\eta}),q_{k,S-r\eta}(\cdot |\tilde{\vx}_{k,r\eta})\right) \le \frac{2\delta^2_0}{n^2_k}\Big| \bigcap_{i=0}^{m_k-1}\left\|\grad\ln p_{k,0}(\vx_i^\prime) - v^\prime_i\right\|\le \delta_1 \right]}_{\text{Lemma B.2}}\right)^{\frac{T}{\eta}\cdot n_k}\\
        & \cdot \left(\sP\left[\bigcap_{i=0}^{m_k-1}\left\|\grad\ln p_{k,0}(\vx_i^\prime) - v^\prime_i\right\|\le \delta_1 \right]\right)^{\frac{T}{\eta}\cdot n_k}\\
        = & (1-2\delta_0)^{\frac{T}{\eta}}\cdot \left(\sP\left[\left\|\grad\ln p_{k,0}(\vx_i^\prime) - v^\prime_i\right\|\le \delta_1\right]\right)^{\frac{T}{\eta}\cdot n_k(\epsilon,-\ln \delta_0)\cdot m_k}
    \end{aligned}
\end{equation*}

To ensure the following inequality is established, 
\begin{equation*}
    \begin{aligned}
        \sP\left[\KL\left(\tilde{q}_{k,S-r\eta}(\cdot |\tilde{\vx}_{k,r\eta}),q_{k,S-r\eta}(\cdot |\tilde{\vx}_{k,r\eta})\right) \le \frac{2\delta^2_0}{n^2_k}\Big| \bigcap_{i=0}^{m_k-1}\left\|\grad\ln p_{k,0}(\vx_i^\prime) - v^\prime_i\right\|\le \delta_1 \right] = 1,
    \end{aligned}
\end{equation*}
Lemma~\ref{lem:inner_err_conv} shows that one of sufficient conditions is  
\begin{equation*}
    \begin{aligned}
        \delta_1 \le L_r \sqrt{2d \tau_r}
    \end{aligned}
\end{equation*}
where the step size of the inner loop $\tau_r$ satisfies
\begin{equation*}
    \tau_r \le \frac{\mu_r}{48L_r^2 d}\cdot \frac{2\delta_0^2}{n_k^2} = \frac{\mu_r}{24 d}\cdot \frac{\delta_0^2}{n_k^2 L_r^2}
\end{equation*}
where follows from Corollary~\ref{cor:kl_conv_inexact_grad}.
In this condition, we have
\begin{equation*}
    \delta_1 \le \sqrt{\frac{\mu_r}{12}}\cdot \frac{\delta_0}{n_k}\le \sqrt{\frac{\mu_r}{12}}\cdot L\epsilon^2 \eta^2\cdot \frac{\delta_0}{\max\left\{d,-\ln \delta_0\right\}}\le \sqrt{\frac{\mu_r}{12}}\cdot \frac{L\epsilon^2\eta^2\delta_0}{d}
\end{equation*}
where we suppose $-\ln \delta_0\le d$ for the last inequality.
Besides, we have
\begin{equation*}
    n_k\ge L^{-1}\epsilon^{-2}\eta^{-2} d\quad \text{and}\quad m_k\ge \frac{2}{\mu_r}\cdot \left(\ln(C_0)+d\right)+\frac{4}{\mu_r}\ln n_k= \frac{2}{\mu_r}\cdot \ln \left(2C_0 \cdot \frac{n_k^2}{2\delta_0^2}\right)=\frac{2}{\mu_r}\cdot \left(\ln(C_0)+2\ln n_k - 2\ln\delta_0\right).
\end{equation*}
It implies the following 
\begin{equation*}
    \sP\left[\bigcap_{k,r} \left\|\grad \ln p_{k,S-r\eta}(\tilde{\vx}_{k,r\eta})-\tilde{\vv}_{k,r\eta}\right\|^2\le 4\epsilon^2\right]\gtrapprox (1-2\delta_0)^{\frac{T}{\eta}} \cdot \left(\sP\left[\left\|\grad\ln p_{k,0}(\vx_i^\prime) - v^\prime_i\right\|\le C_1\cdot \epsilon^2\delta_0 \right]\right)^{\frac{T}{\eta}\cdot  -C_2 \epsilon^{-2}\ln\epsilon}
\end{equation*}
where
\begin{equation*}
    C_1 = \sqrt{\frac{\mu_r}{12}}\cdot \frac{L\eta^2}{d}\quad \text{and}\quad C_2=\frac{4}{\mu_r}.
\end{equation*}
In this proof, the required accuracy of inner loop will exponentially increase, which is not acceptable.

\section{Another Score Estimation Method with OU Process}
\begin{figure}
    \centering
    \input{0_figs/process_explain_3}
    \caption{Recursive Reverse Diffusion Sampling}
    \label{fig:new_sampler_illustration}
\end{figure}
We consider the OU process as the forward process.
\begin{equation}
    \label{eq:ou_sde}
    \der \rvx_t = -\rvx_t \der t + \sqrt{2}\der B_t,\quad \rvx_0\sim p_0 \propto e^{-f_*},
\end{equation}
where the transition kernel satisfies
\begin{equation*}
    p(\vx, t | \vx_0, 0) = \left(2\pi \left(1-e^{-2t}\right)\right)^{-d/2}
     \cdot \exp \left[\frac{-\left\|\vx -e^{-t}\vx_0 \right\|^2}{2\left(1-e^{-2t}\right)}\right], \quad \forall\ 0\le t\le T.
\end{equation*}
Hence, the score function $\grad\ln p_t$ can be reformulated as
\begin{equation*}
    \grad_{\vx} \ln p_{t}(\vx) = \mathbb{E}_{\rvx_0 \sim q_{t}(\cdot|\vx)}\left[-\frac{\vx - e^{-t}\rvx_0}{\left(1-e^{-2t}\right)}\right]
\end{equation*}
where the density function $q_{T-t}(\cdot |\vx)$ is defined as
\begin{equation*}
    q_{t}(\vx_0|\vx) \propto \exp\left(-f_{*}(\vx_0)-\frac{\left\|\vx - e^{-t}\vx_0\right\|^2}{2\left(1-e^{-2t}\right)}\right).
\end{equation*}
It means $q_t$ will be strongly log-concave with a good condition number when 
\begin{equation*}
    L\mI \preceq \grad^2_{\vx^\prime}f_*(\vx^\prime)  + \frac{e^{-2t}}{1-e^{-2t}} \Leftrightarrow t\le \frac{1}{2}\ln\left(\frac{2L+1}{2L}\right).
\end{equation*}
We divide the forward path into several segments whose length is $S=\frac{1}{2}\ln\left(\frac{2L+1}{2L}\right)$.
For each segment, we have
\begin{equation*}
    p_{k,t}(\vx) = \int p_{k,0}(\vx_0)\cdot \mathrm{Pr}\left[\vx, (k,t)| \vx_0, (k,0)\right] \der\vx_0.
\end{equation*}
Similar to the previous derivation, we have
\begin{equation}
    \label{eq:score_est_general}
    \grad\ln p_{k,t}(\vx)=\E_{\rvx^\prime\sim q_{k,t}(\cdot|\vx)}\left[-\frac{\vx - e^{-t}\rvx^\prime}{1-e^{-2t}}\right]\quad \mathrm{where}\quad t\in\left[0,\frac{1}{2}\ln\frac{2L+1}{2L}\right],
\end{equation}
where 
\begin{equation}
    \label{eq:def_aux_dis_general}
    q_{k,t}(\vx^\prime|\vx)\propto \exp\left[-f_{k,0}(\vx^\prime)-\frac{\left\|\vx-e^{-t}\vx^\prime\right\|^2}{2(1-e^{-2t})}\right].
\end{equation}
We need to sample from $q_{k,t}$ to estimate $\grad\ln p_{k,t}$, and the main computational complexity in this process is from the concentration property of $q_{k,t}$.
Different from previous work, here we do not know the explicit form of $f_{k,0}$, hence if we utilize gradient-based MCMC, we need to utilize the recursive method to obtain the score function $\grad\ln q_{k,t}$.
For the gradient-based MCMC, the main computational complexity in this process is from the iterations.
Due to the following fact
\begin{equation*}
    \grad \ln q_{k,t}(\vx^\prime|\vx) = \grad\ln p_{k,0}(\vx^\prime) + \frac{e^{-t}\vx - e^{-2t}\vx^\prime}{1-e^{-2t}},
\end{equation*}
we need to estimate $\grad\ln p_{k,0}$, then we have
\begin{equation*}
    p_{k,0}(\vx) = \int p_{k-1,0}(\vx_0)\cdot \mathrm{Pr}\left[\vx, (k-1,S)| \vx_0, (k-1,0)\right] \der\vx_0.
\end{equation*}
Hence, we have
\begin{equation*}
    \grad\ln p_{k,0}(\vx) = \E_{\rvx^\prime\sim q_{k-1,s}(\cdot|\vx)}\left[-\frac{\vx - e^{-S}\vx^\prime}{1-e^{-2S}}\right],
\end{equation*}
where 
\begin{equation*}
    q_{k-1,S}(\vx^\prime|\vx) \propto \exp\left[-f_{k-1,0}(\vx^\prime) - \frac{\left\|\vx - e^{-s}\vx^\prime\right\|}{2(1-e^{-2s})}\right].
\end{equation*}
Besides, we still utilize ULA to sample $q_{k-1,s}$ whose score function can be obtained by
\begin{equation*}
    \grad\ln q_{k-1,S}(\vx^\prime|\vx)= \grad\ln p_{k-1,0}(\vx^\prime) + \frac{e^{-S}\vx - e^{-2S}\vx^\prime}{1-e^{-2S}}.
\end{equation*}
We summarize the algorithm in Alg~\ref{alg:bpsa}.
Noted that the loop in Line 6 of Alg~\ref{alg:bpsa} is used to estimate the score function $\grad\ln p_{k,S-r\eta}(\tilde{\vx}_{k,r\eta})$ with Eq.~\ref{eq:score_est_general}, and the loop in Line 8 of Alg~\ref{alg:bpsa} is used to sample from $q_{k,S-r\eta}(\cdot|\tilde{\vx}_{k,r\eta})$ with ULA. 
\begin{algorithm}[!hbpt]
    \caption{Reverse Diffusion Sampling}
    \label{alg:bpsa}
    \begin{algorithmic}[1]
            \STATE {\bfseries Input:} Initial particle $\tilde{\vx}_{K,S}$ sampled from $p_\infty$, Terminal time $T$, Step size $\eta$;
            \FOR{$k=K-1$ down to $0$}
                \STATE Initialize the particle as $\tilde{\vx}_{k,0} \coloneqq  \tilde{\vx}_{k+1, S}$;
                \FOR{$r=0$ to $R-1$}
                    \STATE Initialize $\tilde{\vv}_{k,r\eta}=\vzero$;
                    \FOR{$i=1$ to $n_{k,r}$}
                        \STATE Draw $\vx^\prime_{i,0}$ from an initial distribution $q^\prime(\cdot | \tilde{\vx}_{k,r\eta})$
                        \FOR{$j=0$ to $m_{k,r}-1$}
                            \STATE Approximate $\grad\ln p_{k,0}(\vx^\prime_{i,j})$ with $\vv^\prime_j \coloneqq \text{Alg~\ref{alg:sfe_2}}(k,\vx^\prime_{i,j})$;
                            \STATE Update the particle $\vx^\prime_{i,j+1}\coloneqq \vx^\prime_{i,j}+\tau_r \underbrace{\left(\vv^\prime_j + \frac{e^{-(S-r\eta)}\tilde{\vx}_{k,r\eta} - e^{-2(S-r\eta)}\vx^\prime_{i,j}}{1-e^{-2(S-r\eta)}} \right)}_{\text{approximate }\grad\ln q_{k,S-r\eta}(\vx^\prime_{i,j}|\tilde{\vx}_{k,r\eta})} +\sqrt{2\eta}\xi$;
                        \ENDFOR
                        \STATE Update the score estimation with $\tilde{\vv}_{k,r\eta}\coloneqq \tilde{\vv}_{k,r\eta} + \frac{1}{n_{k,r}}\sum_{i=1}^{n_{k,r}}\left[-\frac{\tilde{\vx}_{k,r\eta}-e^{-(S-r\eta)}\vx^\prime_{i,m_{k,r}}}{1-e^{-2(S-r\eta)}}\right]$;
                    \ENDFOR
                    \STATE Update the particle with $\tilde{\vx}_{k, (r+1)\eta} \coloneqq e^\eta\tilde{\vx}_{k,r\eta}+\left(e^\eta - 1\right)\vv_k +\xi$
                \ENDFOR
            \ENDFOR
            \STATE {\bfseries Return:} $\tilde{\vx}_{0,S}$.
    \end{algorithmic}
\end{algorithm}

\begin{algorithm}[!hbpt]
    \caption{Score function estimation (approximate $\grad\ln p_{k,0}(\vx)$)}
    \label{alg:sfe_2}
    \begin{algorithmic}[1]
            \STATE {\bfseries Input:} Segment number $k$, variable $\vx$ requiring the score function;
            \IF{$k\equiv 0$ }
                \STATE {\bfseries Return:} $-\grad f_*(\vx)$. 
            \ENDIF
            \STATE Initial the returned vector $\vv = \vzero$;
            \FOR{$i = 1$ to $n_{k}$}
                \STATE Draw a particle $\vx_0^\prime$ from initial distribution $q^\prime_{0}$;
                \FOR{$j = 0$ to $m_{k}-1$}
                    \STATE Calculate $\vv^\prime_j\approx \grad\ln p_{k-1,0}(\vx_j^\prime)$ by Alg~\ref{alg:sfe_2} with input $(k-1,\vx_j^\prime)$;
                    \STATE Obtain the score by $\grad\ln q_{k-1,S}(\vx^\prime_j | \vx)\approx \Delta_j \coloneqq \vv_j^\prime + \frac{e^{-S}\vx - e^{-2S}\vx^\prime_j}{1-e^{-2S}}$;
                    \STATE Update the particle $\vx_{j+1}^\prime \coloneqq \vx_{j}^\prime + \tau \Delta_j + \sqrt{2\tau}\cdot \xi$
                \ENDFOR
                \STATE Update the score estimation of $\vv\approx \grad\ln p_{k,0}(\vx)$ by $\vv \coloneqq \vv + \frac{1}{n_k}\left[-\frac{\vx - e^{-S}\vx_{mk}^\prime}{1-e^{-2S}}\right]$;
            \ENDFOR
            \STATE {\bfseries Return:} $\vv$.
    \end{algorithmic}
\end{algorithm}
For analysis convenience, we summarize some processes as follows.
The first SDE denotes the forward process.
\begin{equation}
    \label{eq:sde_forward_rev}
    \begin{aligned}
        &\rvx_{0,0}\sim p_{0,0} = p_{*}\quad &\\
        & \der \rvx_{k,t} =-\rvx_{k,t}\der t + \sqrt{2}\der B_{t}\quad &&k\ge 0, t\in[0,S)\\
        &\rvx_{k+1,0}=\rvx_{k,S}\quad && k\ge 0
    \end{aligned}
\end{equation}
We suppose the total time required by the convergence of the forward process, i.e., $T$, satisfies $T/S \in \mathbb{Z}_+$.
Sets $ K\coloneqq T/S$ denoted as the number of segments for the all forward process.


The second SDE denotes the ideal backward process.
\begin{equation}
    \label{eq:sde_backward_ide_rev}
    \begin{aligned}
        &\hat{\rvx}_{K-1,0} \sim p_{K-1,S}\quad &\\
        &\der \hat{\rvx}_{k,t} = \left[\hat{\rvx}_{k,t} + 2\grad\ln p_{k, S-t}(\hat{\rvx}_{k,t})\right]\der t + \sqrt{2}\der B_t\quad && k\in [0,K-1], t\in[0,S)\\
        &\hat{\rvx}_{k-1,0}=\hat{\rvx}_{k,S}\quad && k\in [1,K-1]
    \end{aligned}
\end{equation}
We suppose the length of the segment, i.e., $S$, satisfies $S/\eta \in \mathbb{Z}_+$.
Set $R\coloneqq S/\eta$ denoted as the iteration number of the backward process in each segment.

The third SDE denotes the practical backward process.
\begin{equation}
    \label{eq:sde_backward_act_rev}
    \begin{aligned}
        &\tilde{\rvx}_{K-1,0} \sim p_{\infty, 0}\\
        &\der \tilde{\rvx}_{k,t} = \left[\tilde{\rvx}_{k,t} + 2\tilde{\rvv}_{k, \lfloor t/\eta \rfloor\eta}\left(\tilde{\rvx}_{k, \lfloor t/\eta \rfloor \eta}\right)\right]\der t + \sqrt{2}\der B_t\quad && k\in [0,K-1], t\in[0,S)\\
        &\tilde{\rvx}_{k-1,0}=\tilde{\rvx}_{k,S}\quad && k\in [1,K-1].
    \end{aligned}
\end{equation}





%----------------------------- 

\begin{lemma}
    \label{lem:concen_prop_v2}
    In Alg~\ref{alg:bpsa}, we denote the underlying distribution of output particles as $\rvx_{i,m_{k,r}}\sim q^\prime_{k,S-r\eta}$ which satisfies LSI with the constant $\mu_r^\prime$.
    Then, for any $\vx\in \R^d$, we have
    \begin{equation*}
        \sP\left[\left\|-\frac{1}{n_{k,r}}\sum_{i=1}^{n_{k,r}} \rvx_i^\prime + \E_{\rvx^\prime \sim q^\prime_{k,S-r\eta}(\cdot|\vx)}\left[\rvx^\prime\right]\right\|\le 2\epsilon^\prime\right] \ge 1-\delta
    \end{equation*}
    by requiring the sample number $n_{k,r}(\epsilon^\prime, \delta)$ to satisfy
    \begin{equation*}
        n_{k,r} \ge \frac{1}{\mu_r^\prime \epsilon^{\prime 2}}\max\left\{d, -2\ln \delta\right\}.
    \end{equation*}
\end{lemma}
\begin{proof}
    For any $\vx\in \R^d$, we set
    \begin{equation*}
        \vb^\prime \coloneqq \E_{q^\prime_{k,S-r\eta}(\cdot|\vx)}\left[\rvx^\prime\right]\quad \text{and}\quad  \sigma^\prime\coloneqq \E_{\left\{\rvx^\prime_i\right\}_{i=1}^{n_{k,r}}\sim q^{\prime(n_{k,r})}_{k,S-r\eta}(\cdot|\vx)  }\left[\left\|\sum_{i=1}^{n_{k,r}}\rvx^\prime_i - \E\left[\sum_{i=1}^{n_{k,r}}\rvx^\prime_i\right]\right\|\right].
    \end{equation*}
    Then, considering the following probability
    \begin{equation}
        \begin{aligned}
            &\sP_{\left\{\rvx^\prime_i\right\}_{i=1}^{n_{k,r}}\sim q^{\prime(n_{k,r})}_{k,S-r\eta}(\cdot|\vx)  }\left[\left\|-\frac{1}{n_{k,r}}\sum_{i=1}^{n_{k,r}} \rvx_i^\prime + \E_{\rvx^\prime \sim q^\prime_{k,S-r\eta}(\cdot|\vx)}\left[\rvx^\prime\right]\right\|^2\ge \left(\frac{\sigma^\prime}{n_{k,r}} + \epsilon^\prime\right)^2 \right]\\
            = &  \sP_{\left\{\rvx^\prime_i\right\}_{i=0}^{n_{k,r}-1}\sim q^{\prime(n_{k,r})}_{k,S-r\eta}(\cdot|\vx)  }\left[\left\|\sum_{i=0}^{n_{k,r}-1}\rvx^\prime_i - n_{k,r}\vb^\prime\right\| \ge \sigma^\prime + n_{k,r}\epsilon^\prime\right]
        \end{aligned}
    \end{equation}
    According to previous analysis, we know that $q^\prime_{k,S-r\eta}(\cdot|\vx)$ satisfies LSI with a constant $\mu^\prime_r$ satisfying
    \begin{equation*}
        \mu^\prime_r \ge \frac{e^{-2(S-r\eta)}}{4(1-e^{-2(S-r\eta)})}.
    \end{equation*}
    Combining this result with Lemma~\ref{lem_conv}, we have that the LSI constant of 
    \begin{equation*}
        \sum_{i=0}^{n_{k,r}-1}\rvx_i^\prime \sim \underbrace{q^\prime_{k,S-r\eta}(\cdot|\vx) \ast q^\prime_{k,S-r\eta}(\cdot|\vx) \cdots \ast q^\prime_{k,S-r\eta}(\cdot|\vx)}_{n_{k,r}}
    \end{equation*}
    is $\mu^\prime_r/n_{k,r}$.
    Considering the function $F\left( \vx \right) = \left\| \vx \right\| \colon \R^{d}\rightarrow \R$ is $1$-Lipschitz because
    \begin{equation*}
        \left\|F\right\|_{\mathrm{Lip}}=\sup_{\vx \not= \vy} \frac{\left|F(\vx)-F(\vy)\right|}{\left\|\vx - \vy\right\|}=\sup_{\vx\not = \vy}\frac{\left|\left\| \vx \right\| - \left\| \vy \right\|\right|}{\left\| \left(\vx - \vy \right)\right\|} = 1,
    \end{equation*}
    due to Lemma~\ref{lem:lsi_concentration}, we have 
    \begin{equation*}
        \sP_{\left\{\rvx_i^\prime\right\}_{i=0}^{n_{k,r}-1} \sim q^{\prime(n_{k,r})}_{k,S-r\eta}(\cdot|\vx) }\left[\left\|\sum_{i=0}^{n_{k,r}-1} \rvx_i^\prime- n_{k,r}\vb^\prime \right\|\ge \sigma^\prime + n_{k,r}\epsilon^\prime\right]\le \exp\left(- \frac{\mu^\prime_r \epsilon^{\prime 2} n_{k,r}}{2}\right).
    \end{equation*}
    Besides, we consider the range of $\sigma^\prime$ and have
    \begin{equation*}
        \begin{aligned}
            \sigma^\prime =  & n_{k,r}\cdot \mathbb{E}_{\left\{\rvx_i^\prime\right\}_{i=0}^{n_{k,r}-1} \sim q^{\prime(n_{k,r})}_{k,S-r\eta}(\cdot|\vx)}\left\| \frac{1}{n_{k,r}}\sum_{i=0}^{n_{k,r}-1} \rvx_i^\prime - \vb^\prime\right\|\\
            \le & n_{k,r}\cdot \sqrt{\mathrm{var}\left(\frac{1}{n_{k,r}}\sum_{i=0}^{n_{k,r}-1} \rvx_i^\prime\right)}= \sqrt{n_{k,r} \mathrm{var}\left(\rvx_i^\prime\right)} \le \sqrt{\frac{n_{k,r} d}{\mu^\prime_r}},
        \end{aligned}
    \end{equation*}
    where the first inequality follows from Holder's inequality and the last inequality follows from Lemma~\ref{lem:lsi_var_bound}.
    Hence, we have
    \begin{equation*}
        \sP_{\left\{\rvx^\prime_i\right\}_{i=0}^{n_{k,r}-1}\sim q^{\prime(n_{k,r})}_{k,S-r\eta}(\cdot|\vx)  }\left[\left\|-\frac{1}{n_{k,r}}\sum_{i=0}^{n_{k,r}-1} \rvx_i^\prime + \E_{\rvx^\prime \sim q^\prime_{k,S-r\eta}(\cdot|\vx)}\left[\rvx^\prime\right]\right\|^2\ge \left(\sqrt{\frac{d}{\mu_r^\prime n_{k,r}}} + \epsilon^\prime\right)^2 \right] \le \exp\left(- \frac{\mu^\prime_r \epsilon^{\prime 2} n_{k,r}}{2}\right).
    \end{equation*}
    By requiring 
    \begin{equation}
        \label{ineq:sample_n_req}
        \frac{d}{\mu_r^\prime n_{k,r}} \le \epsilon^{\prime 2} \quad\text{and}\quad -\frac{\mu_r^\prime \epsilon^{\prime 2} n_{k,r}}{2}\le \ln \delta,
    \end{equation}
    we have
    \begin{equation*}
        \begin{aligned}
            &\sP\left[\left\|-\frac{1}{n_{k,r}}\sum_{i=0}^{n_{k,r}-1} \rvx_i^\prime + \E_{\rvx^\prime \sim q^\prime_{k,S-r\eta}(\cdot|\vx)}\left[\rvx^\prime\right]\right\|\le 2\epsilon^\prime\right]\\
            =  & 1- \sP\left[\left\|-\frac{1}{n_{k,r}}\sum_{i=0}^{n_{k,r}-1} \rvx_i^\prime + \E_{\rvx^\prime \sim q^\prime_{k,S-r\eta}(\cdot|\vx)}\left[\rvx^\prime\right]\right\|\ge 2\epsilon^\prime\right] \ge 1- \delta.
        \end{aligned}
    \end{equation*}
    Noted that Eq.~\ref{ineq:sample_n_req} implies the sample number $n_{k,r}$ should satisfy
    \begin{equation*}
        n_{k,r}\ge \frac{d}{\mu_r^\prime\epsilon^{\prime 2}}\quad\text{and}\quad n_{k,r}\ge \frac{2\ln \delta^{-1}}{\mu_r^\prime \epsilon^{\prime 2}}.
    \end{equation*}
    Hence, the proof is completed.
\end{proof}

\begin{lemma}(Lemma 11 in~\cite{vempala2019rapid})
    Suppose $p\propto \exp(-f)$ is $L$-smooth.
    Then, $\E_{p}\left\|\grad f(\rvx)\right\|^2\le Ld$.
\end{lemma}


%--------------------------------------------------
%---------------previous Section B-----------------
\section{Intuitions and Algorithms}
We consider the OU process as the forward process.
\begin{equation}
    \label{eq:ou_sde}
    \der \rvx_t = -\rvx_t \der t + \sqrt{2}\der B_t,\quad \rvx_0\sim p_0 \propto e^{-f_*},
\end{equation}
where the transition kernel satisfies
\begin{equation*}
    p(\vx, t | \vx_0, 0) = \left(2\pi \left(1-e^{-2t}\right)\right)^{-d/2}
     \cdot \exp \left[\frac{-\left\|\vx -e^{-t}\vx_0 \right\|^2}{2\left(1-e^{-2t}\right)}\right], \quad \forall\ 0\le t\le T.
\end{equation*}
Hence, the score function $\grad\ln p_t$ can be reformulated as
\begin{equation*}
    \grad_{\vx} \ln p_{t}(\vx) = \mathbb{E}_{\rvx_0 \sim q_{t}(\cdot|\vx)}\left[-\frac{\vx - e^{-t}\rvx_0}{\left(1-e^{-2t}\right)}\right]
\end{equation*}
where the density function $q_{T-t}(\cdot |\vx)$ is defined as
\begin{equation*}
    q_{t}(\vx_0|\vx) \propto \exp\left(-f_{*}(\vx_0)-\frac{\left\|\vx - e^{-t}\vx_0\right\|^2}{2\left(1-e^{-2t}\right)}\right).
\end{equation*}
It means $q_t$ will be strongly log-concave with a good condition number when 
\begin{equation*}
    \frac{e^{-2t}}{2(1-e^{-2t})}\mI \preceq \grad^2_{\vx^\prime}f_*(\vx^\prime)  + \frac{e^{-2t}}{1-e^{-2t}}\mI \Leftarrow t\le \frac{1}{2}\ln\left(\frac{2L+1}{2L}\right).
\end{equation*}
We divide the forward path into several segments whose length is $S=\frac{1}{2}\ln\left(\frac{2L+1}{2L}\right)$.
For each segment, we have
\begin{equation*}
    p_{k,t}(\vx) = \int p_{k,0}(\vx_0)\cdot \mathrm{Pr}\left[\vx, (k,t)| \vx_0, (k,0)\right] \der\vx_0.
\end{equation*}
Similar to the previous derivation, we have
\begin{equation}
    \label{eq:score_est_general}
    \grad\ln p_{k,t}(\vx)=\E_{\rvx^\prime\sim q_{k,t}(\cdot|\vx)}\left[-\frac{\vx - e^{-t}\rvx^\prime}{1-e^{-2t}}\right]\quad \mathrm{where}\quad t\in\left[0,\frac{1}{2}\ln\frac{2L+1}{2L}\right],
\end{equation}
where 
\begin{equation}
    \label{eq:def_aux_dis_general}
    q_{k,t}(\vx^\prime|\vx)\propto \exp\left[-f_{k,0}(\vx^\prime)-\frac{\left\|\vx-e^{-t}\vx^\prime\right\|^2}{2(1-e^{-2t})}\right].
\end{equation}
We need to sample from $q_{k,t}$ to estimate $\grad\ln p_{k,t}$, and the main computational complexity in this process is from the concentration property of $q_{k,t}$.
Different from previous work, here we do not know the explicit form of $f_{k,0}$ hence, if we utilize gradient-based MCMC, we need to utilize the recursive method to obtain the score function $\grad\ln q_{k,t}$.
For the gradient-based MCMC, the main computational complexity in this process is from the iterations.
Due to the fact
\begin{equation*}
    \grad \ln q_{k,t}(\vx^\prime|\vx) = \grad\ln p_{k,0}(\vx^\prime) + \frac{e^{-t}\vx - e^{-2t}\vx^\prime}{1-e^{-2t}},
\end{equation*}
we need to estimate $\grad\ln p_{k,0}$, then we have
\begin{equation*}
    p_{k,0}(\vx) = \int p_{k-1,0}(\vx_0)\cdot \mathrm{Pr}\left[\vx, (k-1,S)| \vx_0, (k-1,0)\right] \der\vx_0.
\end{equation*}
Hence, we have
\begin{equation*}
    \grad\ln p_{k,0}(\vx) = \E_{\rvx^\prime\sim q_{k-1,s}(\cdot|\vx)}\left[-\frac{\vx - e^{-S}\vx^\prime}{1-e^{-2S}}\right],\quad \text{where}\quad q_{k-1,S}(\vx^\prime|\vx) \propto \exp\left[-f_{k-1,0}(\vx^\prime) - \frac{\left\|\vx - e^{-S}\vx^\prime\right\|^2}{2(1-e^{-2S})}\right].
\end{equation*}
Besides, we still utilize ULA to sample $q_{k-1,s}$ whose score function can be obtained by
\begin{equation*}
    \grad\ln q_{k-1,S}(\vx^\prime|\vx)= \grad\ln p_{k-1,0}(\vx^\prime) + \frac{e^{-S}\vx - e^{-2S}\vx^\prime}{1-e^{-2S}}.
\end{equation*}
We summarize the algorithm in Alg~\ref{alg:bpsa}.
Noted that the loop in Line 6 of Alg~\ref{alg:bpsa} is used to estimate the score function $\grad\ln p_{k,S-r\eta}(\tilde{\vx}_{k,r\eta})$ with Eq.~\ref{eq:score_est_general}, and the loop in Line 8 of Alg~\ref{alg:bpsa} is used to sample from $q_{k,S-r\eta}(\cdot|\tilde{\vx}_{k,r\eta})$ with ULA. 
\begin{algorithm}[!hbpt]
    \caption{Reverse Diffusion Sampling}
    \label{alg:bpsa}
    \begin{algorithmic}[1]
            \State {\bfseries Input:} Initial particle $\tilde{\vx}_{K,S}$ sampled from $p_\infty$, Terminal time $T$, Step size $\eta$;
            \For{$k=K-1$ down to $0$}
                \State Initialize the particle as $\tilde{\vx}_{k,0} \coloneqq  \tilde{\vx}_{k+1, S}$;
                \For{$r=0$ to $R-1$}
                    \State Initialize $\tilde{\vv}_{k,r\eta}=\vzero$;
                    \For{$i=1$ to $n_{k,r}$}
                        \State Draw $\vx^\prime_{i,0}$ from an initial distribution $q^\prime(\cdot | \tilde{\vx}_{k,r\eta})$
                        \For{$j=0$ to $m_{k,r}-1$}
                            \State Approximate $\grad\ln p_{k,0}(\vx^\prime_{i,j})$ with $\vv^\prime_j \coloneqq \text{Alg~\ref{alg:sfe_2}}(k,\vx^\prime_{i,j})$;
                            \State Update the particle $$\vx^\prime_{i,j+1}\coloneqq \vx^\prime_{i,j}+\tau_r \underbrace{\left(\vv^\prime_j + \frac{e^{-(S-r\eta)}\tilde{\vx}_{k,r\eta} - e^{-2(S-r\eta)}\vx^\prime_{i,j}}{1-e^{-2(S-r\eta)}} \right)}_{\text{approximate }\grad\ln q_{k,S-r\eta}(\vx^\prime_{i,j}|\tilde{\vx}_{k,r\eta})} +\sqrt{2\eta}\xi$$
                        \EndFor
                        \State Update the score estimation with $$\tilde{\vv}_{k,r\eta}\coloneqq \tilde{\vv}_{k,r\eta} + \frac{1}{n_{k,r}}\sum_{i=1}^{n_{k,r}}\left[-\frac{\tilde{\vx}_{k,r\eta}-e^{-(S-r\eta)}\vx^\prime_{i,m_{k,r}}}{1-e^{-2(S-r\eta)}}\right]$$
                    \EndFor
                    \State Update the particle with $\tilde{\vx}_{k, (r+1)\eta} \coloneqq e^\eta\tilde{\vx}_{k,r\eta}+\left(e^\eta - 1\right)\vv_k +\xi$
                \EndFor
            \EndFor
            \State {\bfseries Return:} $\tilde{\vx}_{0,S}$.
    \end{algorithmic}
\end{algorithm}

\begin{algorithm}[!hbpt]
    \caption{Score function estimation (approximate $\grad\ln p_{k,0}(\vx)$)}
    \label{alg:sfe_2}
    \begin{algorithmic}[1]
            \State {\bfseries Input:} Segment number $k$, variable $\vx$ requiring the score function;
            \If{$k\equiv 0$ }
                \State {\bfseries Return:} $-\grad f_*(\vx)$. 
            \EndIf
            \State Initial the returned vector $\vv = \vzero$;
            \For{$i = 1$ to $n_{k}$}
                \State Draw a particle $\vx_0^\prime$ from initial distribution $q^\prime_{0}$;
                \For{$j = 0$ to $m_{k}-1$}
                    \State Calculate $\vv^\prime_j\approx \grad\ln p_{k-1,0}(\vx_j^\prime)$ by Alg~\ref{alg:sfe_2} with input $(k-1,\vx_j^\prime)$;
                    \State Obtain the score by $\grad\ln q_{k-1,S}(\vx^\prime_j | \vx)\approx \Delta_j \coloneqq \vv_j^\prime + \frac{e^{-S}\vx - e^{-2S}\vx^\prime_j}{1-e^{-2S}}$;
                    \State Update the particle $\vx_{j+1}^\prime \coloneqq \vx_{j}^\prime + \tau \Delta_j + \sqrt{2\tau}\cdot \xi$
                \EndFor
                \State Update the score estimation of $\vv\approx \grad\ln p_{k,0}(\vx)$ by $\vv \coloneqq \vv + \frac{1}{n_k}\left[-\frac{\vx - e^{-S}\vx_{mk}^\prime}{1-e^{-2S}}\right]$;
            \EndFor
            \State {\bfseries Return:} $\vv$.
    \end{algorithmic}
\end{algorithm}


%---------------------------------------------- Core Calculation ----------------

Hence, we have
    \begin{equation*}
        \small
        \begin{aligned}
            &1+u_{k,r}(10\epsilon)+ u_{k,r}(10\epsilon)\cdot u_{k,0}\left(\frac{10\epsilon}{960}\right)+\ldots + u_{k,r}(10\epsilon)\cdot \prod_{i=k}^2 u_{i,0}\left(\frac{10\epsilon}{960^{k-i+1}}\right)\le (k+1)\cdot u(10\epsilon)\cdot \prod_{i=k}^2 u\left(\frac{10\epsilon}{960^{k-i+1}}\right)\\
            = & (k+1)\cdot u(10\epsilon)\cdot\prod_{i=k}^2 \left(u(10\epsilon)\cdot 960^{k-i+1} \right) = (k+1)\cdot 960^{2.2k(k-1)}\cdot u(10\epsilon)^{k}\le K\cdot 960^{2.2(K-1)(K-2)}\cdot u(10\epsilon)^{K-1}.
        \end{aligned}
    \end{equation*}

\begin{equation*}
        \begin{aligned}
            & \ln \left(960^{2.2(K-1)(K-2)}\cdot u(10\epsilon)^{K-1}\right)= 2.2(K-1)(K-2)\ln(960)+(K-1)\ln(u(10\epsilon)) \\
            \le & 2.2\cdot \ln(960)\cdot \left(\frac{2}{S}\ln \frac{C_0}{\epsilon}\right)^2+ \frac{2}{S}\ln \frac{C_0}{\epsilon}\cdot \left(\ln\frac{C_nC_m}{10^{4.4}}+\ln\frac{1}{\epsilon^{4.4}}\right)\\
            \le & \frac{55}{S^2}\left(\ln \frac{C_0}{\epsilon}\right)^2+ \frac{2}{S}\ln \frac{C_0}{\epsilon}\cdot\left[\ln\left(2^{11.2}\cdot 3^{2}C_0^{0.2}C_1^{-2.2}\cdot (d+m_2^2)^{2.2}d\cdot \max\{d, -2\ln \delta\}\right)+\ln(\epsilon^{-4.4})\right]\\
            \le & \frac{55}{S^2}\left(\ln \frac{C_0}{\epsilon}\right)^2+ \frac{2}{S}\ln \frac{C_0}{\epsilon}\cdot \left(33+0.2\ln C_0+4.4\ln L + 3.2\ln (d+m_2^2)+\ln\ln\frac{1}{\delta} +4.4\ln \frac{1}{\epsilon}\right),
        \end{aligned}
    \end{equation*}
    which means
    \begin{equation}
        \label{ineq:grad_comp_cal}
        \begin{aligned}
            & 960^{2.2(K-1)(K-2)}\cdot u(10\epsilon)^{K-1}\\
            \le & \exp\left(\frac{55}{S^2}\left(\ln \frac{C_0}{\epsilon}\right)^2+ \frac{2}{S}\ln \frac{C_0}{\epsilon}\cdot \left(33+0.2\ln C_0+4.4\ln L + 3.2\ln (d+m_2^2)+\ln\ln\frac{1}{\delta} +4.4\ln \frac{1}{\epsilon}\right)\right)\\
            \le & C_2\cdot \epsilon^{-\frac{55}{S^2}\ln \frac{C_0^2}{\epsilon}}\cdot C_3\cdot \epsilon^{-\frac{2}{S}\left(33+4.6\ln C_0 + 4.4\ln L + 4.4\ln \frac{1}{\epsilon}\right)}\cdot (d+m_2^2)^{\frac{6.4}{S}\ln \frac{C_0}{\epsilon}}\cdot (\ln(1/\delta))^{\frac{2}{S}\ln \frac{C_0}{\epsilon}},
        \end{aligned}
    \end{equation}
    where the last inequality needs careful algebra calculation.
    Noted that $C_2$ and $C_3$ are constant independent with $\epsilon$, $d$ and $\delta$ defined as follows
    \begin{equation*}
        C_2=C_0^{-\frac{55}{S^2}\ln C_0} \quad \mathrm{and}\quad C_3=C_0^{\frac{2}{S}\left(33+0.2\ln C_0+ 4.4\ln L\right)}.
    \end{equation*}
    Plugging this result into Eq~\ref{ineq:prob_lob_mid}, we have
    \begin{equation}
        \label{ineq:prob_lob_mid2}
        \begin{aligned}
            &\sP\left[\left\|\grad\ln p_{k,S-r\eta}(\vx)- \tilde{\rvv}_{k,r\eta}(\vx)\right\|^2\le 10\epsilon,\forall \vx\in\R^d\right]\\
            \ge & 1-\delta \cdot K\cdot C_2C_3\cdot \epsilon^{-\frac{2}{S}\left(33+0.2\ln C_0 + 4.4\ln L\right)-\frac{8.8}{S}\ln \frac{C_0}{\epsilon}-\frac{55}{S^2}\ln \frac{C_0^2}{\epsilon}} \cdot (d+m_2^2)^{\frac{6.4}{S}\ln \frac{C_0}{\epsilon}}\cdot \left(-\ln {\delta}\right)^{\frac{2}{S}\ln\frac{C_0}{\epsilon}}.
        \end{aligned}
    \end{equation}

    With these conditions, we are able to lower bound score estimation errors along Alg~\ref{alg:bpsa}. 
    That is
    \begin{equation*}
        \begin{aligned}
           & \sP\left[\bigcap_{
                \substack{k\in \mathbb{N}_{0,K-1}\\ r\in\mathbb{N}_{0,R-1}}
           }\left\|\grad\ln p_{k,S-r\eta}(\tilde{\vx}_{k,r\eta})-\tilde{\rvv}_{k,r\eta}(\tilde{\vx}_{k,r\eta})\right\|^2\le 10\epsilon\right]\\
           = & \prod_{
                \substack{k\in \mathbb{N}_{0,K-1}\\ r\in\mathbb{N}_{0,R-1}}
           } \sP\left[\left\|\grad\ln p_{k,S-r\eta}(\tilde{\vx}_{k,r\eta})-\tilde{\rvv}_{k,r\eta}(\tilde{\vx}_{k,r\eta})\right\|^2\le 10\epsilon\right]\\
           \ge & \prod_{
                \substack{k\in \mathbb{N}_{0,K-1}\\ r\in\mathbb{N}_{0,R-1}}
           } \sP\left[\left\|\grad\ln p_{k,S-r\eta}(\vx)- \tilde{\rvv}_{k,r\eta}(\vx)\right\|^2\le 10\epsilon,\forall \vx\in\R^d\right]
        \end{aligned}
    \end{equation*}
    where the first inequality establishes because the random variables, $\tilde{\rvv}_{k,r\eta}$, are independent for each $(k,r)$ pair.
    By introducing Eq~\ref{ineq:prob_lob_mid2}, we have
    \begin{equation}
        \small
        \label{ineq:prob_lob_mid3}
        \begin{aligned}
            &\prod_{
                \substack{k\in \mathbb{N}_{0,K-1}\\ r\in\mathbb{N}_{0,R-1}}
           } \sP\left[\left\|\grad\ln p_{k,S-r\eta}(\vx)- \tilde{\rvv}_{k,r\eta}(\vx)\right\|^2\le 10\epsilon,\forall \vx\in\R^d\right]\\
           \ge & \left(1-\delta \cdot K\cdot C_2C_3\cdot \epsilon^{-\frac{2}{S}\left(33+0.2\ln C_0 + 4.4\ln L\right)-\frac{8.8}{S}\ln \frac{C_0}{\epsilon}-\frac{55}{S^2}\ln \frac{C_0^2}{\epsilon}} \cdot (d+m_2^2)^{\frac{6.4}{S}\ln \frac{C_0}{\epsilon}}\cdot \left(-\ln {\delta}\right)^{\frac{2}{S}\ln\frac{C_0}{\epsilon}}\right)^{KR}\\
           \ge & 1- \delta\cdot K^2R\cdot C_2C_3\cdot \epsilon^{-\frac{2}{S}\left(33+0.2\ln C_0 + 4.4\ln L\right)-\frac{8.8}{S}\ln \frac{C_0}{\epsilon}-\frac{55}{S^2}\ln \frac{C_0^2}{\epsilon}} \cdot (d+m_2^2)^{\frac{6.4}{S}\ln \frac{C_0}{\epsilon}}\cdot \left(-\ln {\delta}\right)^{\frac{2}{S}\ln\frac{C_0}{\epsilon}}\\
           = & 1- \delta\cdot  \frac{4(d+m_2^2)}{SC_1\epsilon}\left(\ln \frac{C_0}{\epsilon}\right)^2\cdot C_2C_3\cdot \epsilon^{-\frac{2}{S}\left(33+0.2\ln C_0 + 4.4\ln L\right)-\frac{8.8}{S}\ln \frac{C_0}{\epsilon}-\frac{55}{S^2}\ln \frac{C_0^2}{\epsilon}} \cdot (d+m_2^2)^{\frac{6.4}{S}\ln \frac{C_0}{\epsilon}}\cdot \left(-\ln {\delta}\right)^{\frac{2}{S}\ln\frac{C_0}{\epsilon}}
        \end{aligned}
    \end{equation}
    where the first inequality follows from Eq~\ref{ineq:prob_lob_mid2} and the second inequality follows from the union bound, and the last inequality follows from the combination of the choice of the step size, i.e., $\eta=C_1(d+m_2^2)^{-1}\epsilon$ and the definition of $K$ and $R$, i.e.,
    \begin{equation*}
        K=\frac{T}{S}= \frac{2}{S}\ln\frac{C_0}{\epsilon},\quad R=\frac{S}{\eta}=\frac{S(d+m_2^2)}{C_1\epsilon}.
    \end{equation*}
    
    It means when $\delta$ is small enough, we can control the recursive error with a high probability, i.e.,
    \begin{equation}
        \label{ineq:prob_lob_mid4}
        \prod_{
                \substack{k\in \mathbb{N}_{0,K-1}\\ r\in\mathbb{N}_{0,R-1}}
           } \sP\left[\left\|\grad\ln p_{k,S-r\eta}(\vx)- \tilde{\rvv}_{k,r\eta}(\vx)\right\|^2\le 10\epsilon,\forall \vx\in\R^d\right]\ge 1-\epsilon.
    \end{equation}
    Compared with Eq~\ref{ineq:prob_lob_mid3}, Eq~\ref{ineq:prob_lob_mid4} can be achieved by requiring
    \begin{equation}
        \label{ineq:delta_req}
        C_B\delta (-\ln \delta)^{\frac{2}{S}\ln \frac{C_0}{\epsilon}}\le \epsilon\quad \Leftrightarrow\quad (-\ln \delta)^{\frac{2}{S}\ln \frac{C_0}{\epsilon}}\le \frac{\epsilon}{C_B \delta} \quad \Leftrightarrow\quad \frac{2}{S}\ln \frac{C_0}{\epsilon}\cdot \ln\ln\frac{1}{\delta}\le \ln \frac{\epsilon}{ C_B \delta}
    \end{equation}
    where 
    \begin{equation*}
        C_B \coloneqq  \frac{4(d+m_2^2)}{SC_1\epsilon}\left(\ln \frac{C_0}{\epsilon}\right)^2\cdot C_2C_3\cdot \epsilon^{-\frac{2}{S}\left(33+0.2\ln C_0 + 4.4\ln L\right)-\frac{8.8}{S}\ln \frac{C_0}{\epsilon}-\frac{55}{S^2}\ln \frac{C_0^2}{\epsilon}} \cdot (d+m_2^2)^{\frac{6.4}{S}\ln \frac{C_0}{\epsilon}}.
    \end{equation*}
    We suppose $\delta=\epsilon/C_B\cdot a^{-2/S\cdot \ln (C_0/\epsilon)}$ and the last inequality of Eq~\ref{ineq:delta_req} becomes
    \begin{equation*}
        \begin{aligned}
            &\mathrm{LHS}= \frac{2}{S}\ln \frac{C_0}{\epsilon}\cdot \ln\left[\ln\frac{C_B}{\epsilon}+\frac{2}{S}\ln\frac{C_0}{\epsilon}\cdot \ln a\right]\le  \frac{2}{S}\ln \frac{C_0}{\epsilon}\cdot\ln a = \mathrm{RHS},
        \end{aligned}
    \end{equation*}
    which is hold if we require 
    \begin{equation*}
        a\ge \max\left\{\frac{2C_B}{\epsilon}, \left(\frac{C_0}{\epsilon}\right)^{2/S},1\right\}.
    \end{equation*}
    Because in this condition, we have
    \begin{equation*}
        \begin{aligned}
            \ln \frac{C_B}{\epsilon}+\frac{2}{S}\ln \frac{C_0}{\epsilon}\cdot \ln a\le  \ln \frac{a}{2}+ (\ln a)^2 \le  \frac{2a}{5}+\frac{3a}{5}=a\quad \mathrm{when}\quad a\ge 1,
        \end{aligned}
    \end{equation*}
    where the first inequality follows from the monotonicity of function $\ln(\cdot)$. 
    Therefore, we have
    \begin{equation*}
        \ln\left[\ln\frac{C_B}{\epsilon}+\frac{2}{S}\ln\frac{C_0}{\epsilon}\cdot \ln a\right]\le \ln a
    \end{equation*}
    and Eq~\ref{ineq:delta_req} establishes. 
    Without loss of generality, we suppose $3C_B/\epsilon$ dominates the lower bound of $a$. 
    Hence, the choice of $\delta$ can be determined.

    After determining the choice of $\delta$, the only problem left is the gradient complexity of Alg~\ref{alg:bpsa}.
    The number of gradients calculated in Alg~\ref{alg:bpsa} is equal to the number of calls
    for $\tilde{\rvv}_{-1,0}$.
    According to Eq~\ref{ineq:prob_lob_mid}, we can easily note that the number of calls of $\tilde{\rvv}_{-1,0}$ is 
    \begin{equation*}
        u_{k,r}(10\epsilon)\cdot \prod_{i=k}^1 u_{i,0}\left(\frac{10\epsilon}{960^{k-i+1}}\right) = u(10\epsilon)\prod_{i=k}^1 u\left(\frac{10\epsilon}{960^{k-i+1}}\right)
    \end{equation*}
    for each $(k,r)$ pair. 
    We can upper bound RHS of the previous equation as
    \begin{equation*}
        \begin{aligned}
            & u(10\epsilon)\prod_{i=k}^1 u\left(\frac{10\epsilon}{960^{k-i+1}}\right)= u(10\epsilon)\cdot\prod_{i=k}^2 \left(u(10\epsilon)\cdot 960^{k-i+1} \right)\\
            = & 960^{2.2k(k-1)}\cdot u(10\epsilon)^{k} \le 960^{2.2(K-1)(K-2)}\cdot u(10\epsilon)^{K-1}
        \end{aligned}
    \end{equation*}
    Combining this result with the total number of $(k,r)$ pair, i.e., $T/\eta$, the total gradient complexity can be relaxed as
    \begin{equation}
        \label{ineq:grad_comp_fin1}
        \begin{aligned}
            & \frac{T}{\eta} \cdot 960^{2.2k(k-1)}\cdot u(10\epsilon)^{k} \le K^2R\cdot 960^{2.2(K-1)(K-2)}\cdot u(10\epsilon)^{K-1}\\
            \le & \frac{4(d+m_2^2)}{SC_1\epsilon}\left(\ln \frac{C_0}{\epsilon}\right)^2\cdot C_2C_3\cdot \epsilon^{-\frac{2}{S}\left(33+0.2\ln C_0 + 4.4\ln L\right)-\frac{8.8}{S}\ln \frac{C_0}{\epsilon}-\frac{55}{S^2}\ln \frac{C_0^2}{\epsilon}} \cdot (d+m_2^2)^{\frac{6.4}{S}\ln \frac{C_0}{\epsilon}}\cdot \left(-\ln {\delta}\right)^{\frac{2}{S}\ln\frac{C_0}{\epsilon}}\\
            = & C_B\cdot (-\ln \delta)^{\frac{2}{S}\ln \frac{C_0}{\epsilon}} \le \frac{\epsilon}{\delta} = C_B\cdot a^{\frac{2}{S}\ln \frac{C_0}{\epsilon}}
        \end{aligned}
    \end{equation}
    where the first inequality follows from the fact $T/\eta = KR$, the second inequality follows from the combination of the choice of the step size, i.e., $\eta=C_1(d+m_2^2)^{-1}\epsilon$ and the definition of $K$ and $R$, i.e.,
    \begin{equation*}
        K=\frac{T}{S}= \frac{2}{S}\ln\frac{C_0}{\epsilon},\quad R=\frac{S}{\eta}=\frac{S(d+m_2^2)}{C_1\epsilon}
    \end{equation*}
    and the last inequality follows from~\ref{ineq:delta_req}.
    Choosing $a$ as its lower bound, i.e., $2C_B/\epsilon$, RHS of Eq~\ref{ineq:grad_comp_fin1} satisfies
    \begin{equation*}
        \label{ineq:grad_comp_fin2}
        \begin{aligned}
            & C_B\cdot a^{\frac{2}{S}\ln \frac{C_0}{\epsilon}} = C_B \cdot \left(\frac{2C_B}{\epsilon}\right)^{\frac{2}{S}\ln \frac{C_0}{\epsilon}}\le \left(\frac{2C_B}{\epsilon}\right)^{\frac{4}{S}\ln \frac{C_0}{\epsilon}}\\
            \le & \left(\frac{8(d+m_2^2)}{S C_1\epsilon^2}\cdot \left(\frac{C_0}{\epsilon}\right)^2\right)^{\frac{4}{S}\ln\frac{C_0}{\epsilon}}\cdot \left(C_2C_3\right)^{\frac{4}{S}\ln\frac{C_0}{\epsilon}}\cdot (d+m_2^2)^{\frac{26}{S^2} \left(\ln \frac{C_0}{\epsilon}\right)^2}\\
            & \cdot \epsilon^{-\frac{8}{S^2}\left(33+0.2\ln C_0 + 4.4\ln L\right)\cdot \ln \frac{C_0}{\epsilon}-\left(\frac{36}{S^2}+ \frac{252}{S^3}\right)\cdot \left(\ln \frac{C_0}{\epsilon}\right)^2}\\
            = & C_0^{\frac{4}{S}\ln \frac{8C_0C_2C_3}{SC_1}}\cdot (d+m_2^2)^{\frac{4}{S}\cdot \ln \frac{C_0}{\epsilon}+ \frac{26}{S^2}\cdot  \left(\ln \frac{C_0}{\epsilon}\right)^2}\\
            & \cdot \epsilon^{-\frac{4}{S}\ln \frac{8C_0^2}{SC_1} -\left(\frac{8}{S^2}\left(33+0.2\ln C_0 + 4.4\ln L\right)+\frac{16}{S}\right)\cdot \ln \frac{C_0}{\epsilon}-\left(\frac{36}{S^2}+ \frac{252}{S^3}\right)\cdot \left(\ln \frac{C_0}{\epsilon}\right)^2 }\\
            = & \mathrm{poly}\left(\frac{d+m_2^2}{\epsilon},  \ln \frac{1}{\epsilon}\right)
        \end{aligned}
    \end{equation*}
    Hence, the proof is completed.

    \begin{table}[b]
        \centering
        \begin{tabular}{c|c|c|c}
             Gradient complexity& ULA~\cite{neal1992bayesian} & DMC~\cite{huang2023monte} & RS-DMC \\
             \hline
             200 & $1.386$ & $1.009\times 10^{-1}$ & $8.716\times10^{-2}$\\
             \hline
             400  & $1.386$ & $8.776\times 10^{-2}$ & $7.427\times 10^{-2}$\\
             \hline
             800 & $1.386$ & $7.957\times 10^{-2}$ & $5.700\times 10^{-2}$\\
             \hline 
             1600 & $1.382$ & $7.777 \times 10^{-2}$ & $4.430 \times 10^{-2}$ \\
             \hline
             3200 & $1.382$ & $6.045 \times 10^{-2}$ & $3.758\times 10^{-2}$\\
             \hline
        \end{tabular}
        \caption{Exact MMD values for ULA, DMC, and RS-DMC for the different gradient complexity}
        \label{tab:exp_mmd}
    \end{table}
